# Supplementary material for: Professional Differences: A Comparative Study of Visualization Task Performance and Spatial Ability Across Disciplines
Source: arXiv:2108.02333 ancillary file (2021-08-05)
Supplement: Supplementary file 1 [file DemographicsSupplement.pdf]

# Demographic & Educational Analysis Supplement

**Professional Differences: A Comparative Study of Visualization Task Performance and Spatial Ability Across Disciplines**

IEEE VIS 2021

Kyle Hall, Anthony Kouroupis, Anastasia Bezerianos, Danielle Albers Szafir, and Christopher Collins

The following analyses are based on the files “degrees 2020-03-30.csv” and “demographic_2020-03-30_EdAnalysis.csv”, which are located under Quantitative Analysis Supplement/Data of Supplemental Materials. The *HighestDegree* and *DegreeInProgress* fields in “demographic_2020-03-30_EdAnalysis.csv” were created by manually inspecting the degree information in “degrees 2020-03-30.csv”.

## Demographic Distributions

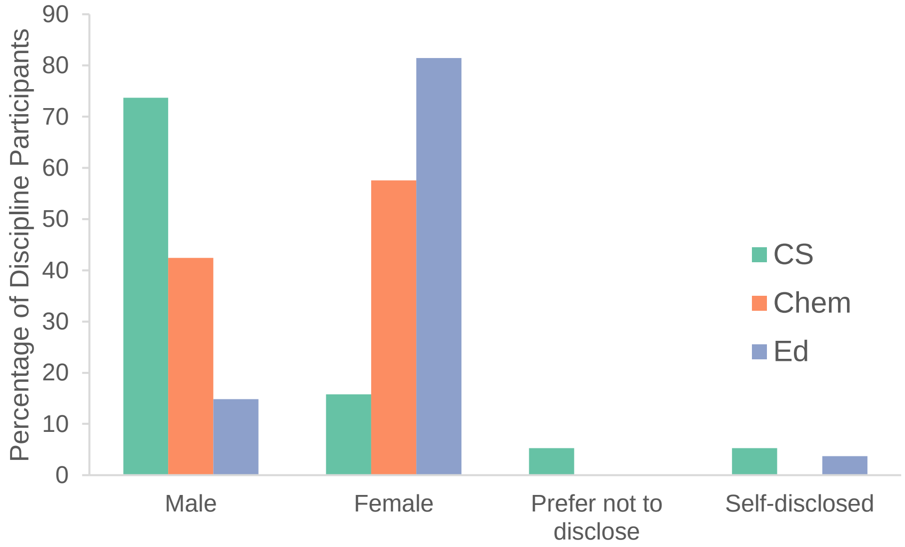


**Figure S1.** Gender distribution of participants from the three disciplines considered in this study: Computer Science (CS), Chemistry and Education. Participants had the options to select *Female*, *Male*, *Prefer not to disclose*, or self-disclose another option as a free-form string.

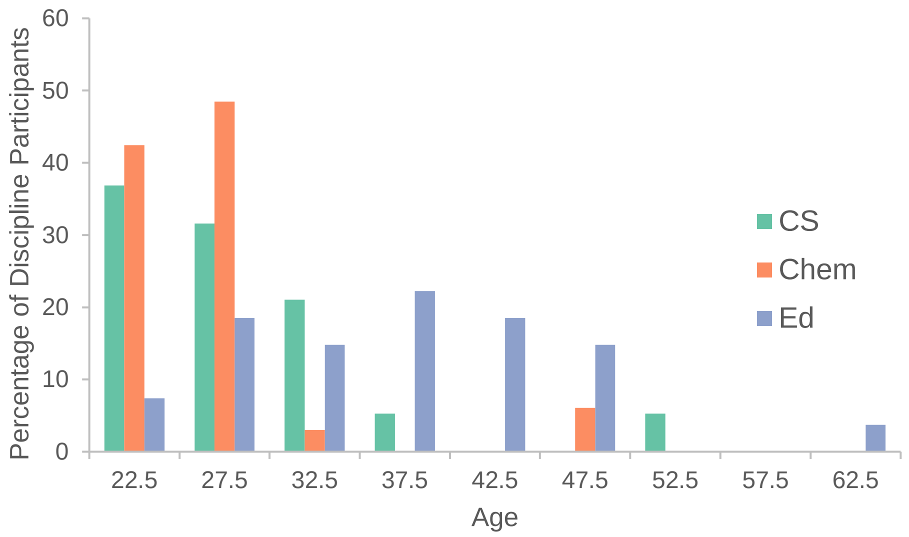


**Figure S2.** Histograms of the age distribution of participants from the three disciplines considered in this study. The histograms were constructed using a bin width of 5 years. The minimum and maximum ages of participants were 21 and 64.

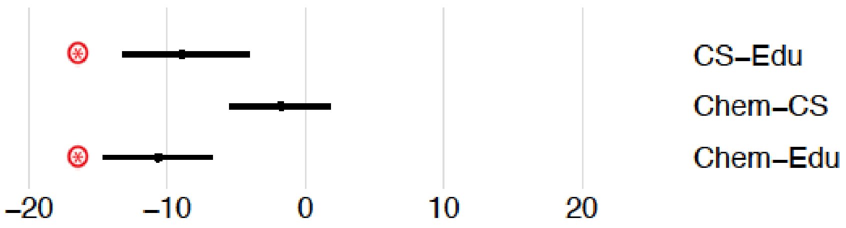


**Figure S3.** The Confidence Intervals of mean differences for age. CI estimation techniques show no evidence of a difference between CS and Chemistry, but Education ages tend to be older.

## Analysis of Education Histories

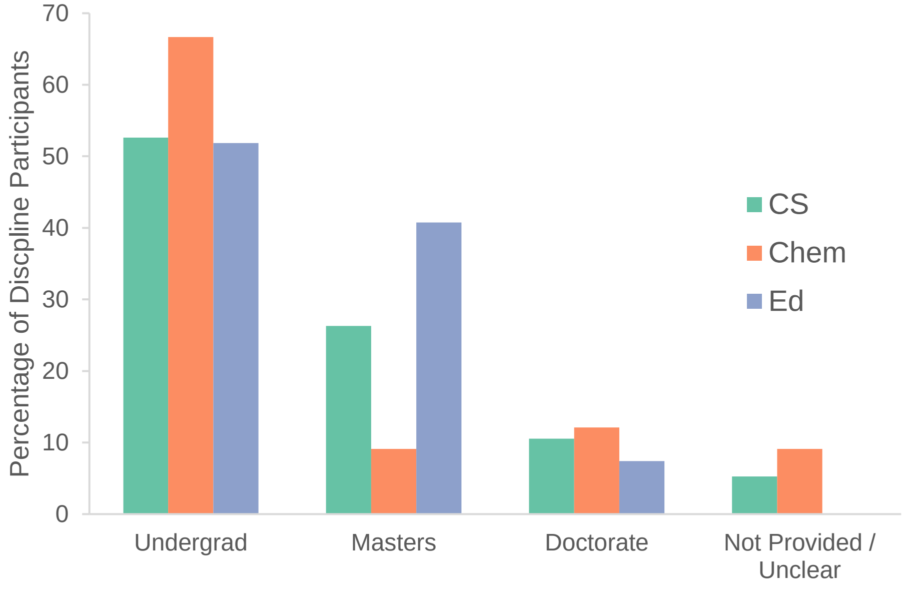


**Figure S4.** Distribution of highest level of education attainment across the disciplines. All "Bachelor" related degrees (e.g., BA, BEd, and Bachelor of Science) were labeled undergraduate for the purpose of this analysis. When reporting education information, participants had to indicate whether degrees were *complete* or *in progress.* The attainment statistics are also based only on those degrees that participants reported as being *complete*. See Figure S5 for statistics about degrees *in progress*.

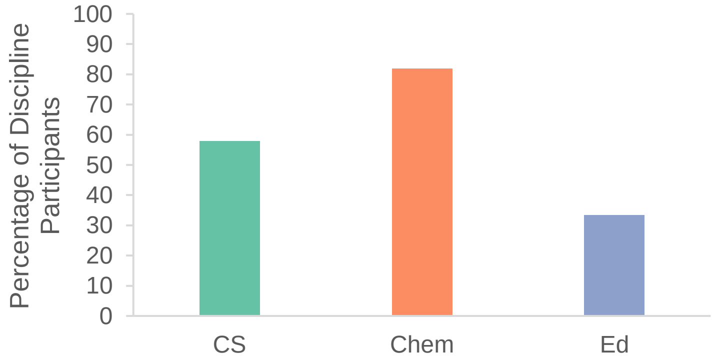


**Figure S5.** Percentages of participants with degrees in progress. When reporting education information, participants had to indicate whether degrees were *complete* or *in progress.* We did have one individual indicate that they were currently completing multiple education training programs.

**Undergraduate Education Analysis for Education Participants**

Analysis of the educational information for the participants who self-identified as educators revealed that 18% of our education participants (5 participants) had educational histories with degrees potentially related to computer science (e.g., Information Technology, Educational Technology, and a minor in Computer Science), and 22% of participants (6 individuals) reported undergraduate degrees in STEM (e.g., Mathematics and Health). We had additional participants from the humanities and social sciences (e.g., French, English and Religious Studies) and the arts (e.g., Painting and Music). None of our education participants appeared to have a chemistry background, though 3 education participants did not provide their undergraduate degree information. However, 37% of participants (10 individuals) specifically indicated that their undergraduate degree was in an education-related field (e.g., Early Childhood Education and Child & Youth Care). These results suggest that there is a sizable contingent of individuals for whom their primary post-secondary training was in education.

For this analysis, we reviewed all degrees held by education participants that had titles that could related to undergraduate degrees (e.g., Bachelors, Bachelor of Science and BA). For the purposes of revealing professional intersections, we filter the undergraduate degrees by selecting only those undergraduate degrees that were non-education degrees (i.e., BSc vs. BEd) unless a participant only had one reported undergraduate and it was in education (e.g., *Early Childhood Education*). Note that some education participants did not provide their undergraduate information. Based on the resulting filtered list, we assigned people as have either a primary undergraduate degree in STEM or Education as detailed below. The outcome of this process is provided in Table S1 where readers can find additional information about the undergraduate degrees of education participants.

**Table S1.** The undergraduate specialization for participants from education. A semi-colon is used to separate degree areas when a participant had multiple undergraduate degrees outside education.

| id | sessionid | Undergraduate Specialization | Undergraduate Degree in STEM | Undergraduate Degree in Ed. |
|---:|---:|---|---|---|
| 118 | 129382 | French | No | No |
| 115 | 133269 | General Studies | No | No |
| 113 | 137930 | History; Religious Studies | No | No |
| 60 | 185465 | Early Childhood Education | No | Yes |
| 116 | 224364 | Child and Youth Care | No | Yes |
| 57 | 309678 | Health | Yes | No |
| 112 | 400716 | Primary/Junior/Intermediate/Senior | No | Yes |
| 102 | 412490 | BFA (Painting) | No | No |
| 101 | 457768 | Not Provided | N/A | N/A |
| 56 | 487261 | English Literature | No | No |
| 75 | 487731 | Elementary Education | No | Yes |
| 121 | 551790 | English / Religious Studies | No | No |
| 76 | 586515 | English Literature, minor in computer science | Yes | No |
| 108 | 589143 | Religious Studies/Women's Studies; Trumpet Performance | No | No |
| 55 | 603798 | Child & Youth Care | No | Yes |

| | | | | |
|---|---|---|---|---|
| 89 | 665822 | Physical Education | No | Yes |
| 120 | 694511 | Cognitive Science | Yes | No |
| 93 | 703754 | Early Childhood Education | No | Yes |
| 117 | 764411 | Mathematics | Yes | No |
| 111 | 803014 | Neuroscience, Physiology, and Forest Conservation Science | Yes | No |
| 79 | 810153 | Film | No | No |
| 54 | 827935 | Education | No | Yes |
| 114 | 843435 | Child and Youth Studies | No | Yes |
| 124 | 851243 | Elementary education K-6 | No | Yes |
| 78 | 931997 | Not provided | N/A | N/A |
| 77 | 949909 | Not provided | N/A | N/A |
| 123 | 999085 | Pure Mathematics/Computer Science | Yes | No |
