# Supplementary material for: Professional Differences: A Comparative Study of Visualization Task Performance and Spatial Ability Across Disciplines
Source: arXiv:2108.02333 ancillary file (2021-08-05)
Supplement: Supplementary file 2 [file Qualitative_Coding_Supplement.pdf]

# Professional Differences: A Comparative Study of Visualization Task Performance and Spatial Ability Across Disciplines

## Qualiative Data Supplement
## IEEE VIS 2021

Kyle Hall, Anthony Kouroupis, Anastasia Bezerianos, Danielle Albers Szafir, and Christopher Collins

| Summary by Task | | | | | |
|---|---|---|---|---|---|
| **Strategies** | **Code** | **Description** | **Mean % CS by task** | **Mean % Chemisty by task** | **Mean % Education** |
| | s-s | specific – describe a specific strategy that may or may not be discretized that could inform another person in creating his/her own strategy. Strategy is potentially reproducible | **0.118** | **0.144** | **0.058** |
| | s-d | discreet steps, the same step repeated | **0.211** | **0.091** | **0.202** |
| | s-p | used prop/hand/external aid | **0.066** | **0.061** | **0.144** |
| | s-t | skill transference, metaphor usage (mapping) | **0.039** | **0.045** | **0.000** |
| | s-m | nonspecific mental visualization (e.g. "imagined it", "visualized it") | **0.184** | **0.159** | **0.192** |
| | s-i | using interaction | **0.211** | **0.235** | **0.192** |
| | s-o | following an ordered approach (e.g. small to large; faces in sequence) | **0.079** | **0.045** | **0.048** |
| | q | mentioned difficulty, confusion | **0.013** | **0.015** | **0.096** |
| | s-u | strategy as described is unclear | **0.132** | **0.098** | **0.106** |
| | s-e | followed a process of elimination | **0.013** | **0.038** | **0.010** |
| | s-a | rapidly alternating between views | **0.000** | **0.030** | **0.038** |
| | s-y | Symmetry – discussed symmetry concept (e.g., reflection, rotation, or discussions of symmetry related concepts: handedness, chiral, stereo) | **0.000** | **0.045** | **0.029** |
| | s-r | Mirror – mentioned the mirror image relationship of opposite sides. Note that mirror is special case of the symmetry label. | **0.013** | **0.053** | **0.000** |
| | | | | | |
| **Generated Landmarks** | g-axes | using axes to navigate task (when axes are not present); note in PSVT there were no axes provided | **0.000** | **0.030** | **0.000** |
| | g-ref | using generated reference points such as characteristic angles (e.g., 90 deg) or creating groups of angles | **0.000** | **0.061** | **0.019** |
| | | | | | |
| **Visual Landmarks** | v-u | using a unique component, corner, edge, or face for reference | **0.066** | **0.114** | **0.038** |
| | v-z | unspecified mention of size | **0.066** | **0.045** | **0.029** |
| | v-r | using area to compare sizes | **0.000** | **0.008** | **0.000** |
| | v-a | using angle or arc to compare sizes | **0.066** | **0.076** | **0.029** |
| | v-o | Outlier – used outliers/maxima/minima to perform task | **0.105** | **0.114** | **0.135** |
| | v-c | Cluster – analyzed points in terms of groups | **0.039** | **0.045** | **0.010** |
| | v-x | using visual axes to assist in the task | **0.184** | **0.174** | **0.096** |
| | v-s | using a shape feature (valley, shoulder, contour) | **0.039** | **0.053** | **0.010** |
| | v-h | used specific colors (hues) to make decision | **0.079** | **0.076** | **0.096** |

| Category | | | 1.000 | 2.000 | 3.000 |
|---|---|---|---|---|---|
| **Strategies** | **Code** | **Description** | **% CS mentioned at least once** | **% Chemistry mentioned at least once** | **% Education mentioned at least once** |
| | s-s | specific – describe a specific strategy that may or may not be discretized that could inform another person in creating his/her own strategy. Strategy is potentially reproducible | 0.421 | 0.424 | 0.192 |
| | s-d | discreet steps, the same step repeated | 0.579 | 0.333 | 0.615 |
| | s-p | used prop/hand/external aid | 0.263 | 0.212 | 0.500 |
| | s-t | skill transference, metaphor usage (mapping) | 0.105 | 0.121 | 0.000 |
| | s-m | nonspecific mental visualization (e.g. "imagined it", "visualized it") | 0.474 | 0.394 | 0.423 |
| | s-i | using interaction | 0.579 | 0.758 | 0.500 |
| | s-o | following an ordered approach (e.g. small to large; faces in sequence) | 0.263 | 0.182 | 0.192 |
| | q | mentioned difficulty, confusion | 0.053 | 0.061 | 0.269 |
| | s-u | strategy as described is unclear | 0.316 | 0.273 | 0.346 |
| | s-e | followed a process of elimination | 0.053 | 0.152 | 0.038 |
| | s-a | rapidly alternating between views | 0.000 | 0.121 | 0.154 |
| | s-y | Symmetry – discussed symmetry concept (e.g., reflection, rotation, or discussions of symmetry related concepts: handedness, chiral, stereo) | 0.000 | 0.182 | 0.115 |
| | s-r | Mirror – mentioned the mirror image relationship of opposite sides. Note that mirror is special case of the symmetry label. | 0.053 | 0.212 | 0.000 |
| | | | | | |
| **Generated Landmarks** | g-axes | using axes to navigate task (when axes are not present); note in PSVT there were no axes provided | 0.000 | 0.121 | 0.000 |
| | g-ref | using generated reference points such as characteristic angles (e.g., 90 deg) or creating groups of angles | 0.000 | 0.242 | 0.077 |
| | | | | | |
| **Visual Landmarks** | v-u | using a unique component, corner, edge, or face for reference | 0.211 | 0.364 | 0.154 |
| | v-z | unspecified mention of size | 0.263 | 0.182 | 0.115 |
| | v-r | using area to compare sizes | 0.000 | 0.030 | 0.000 |
| | v-a | using angle or arc to compare sizes | 0.263 | 0.303 | 0.115 |
| | v-o | Outlier – used outliers/maxima/minima to perform task | 0.421 | 0.364 | 0.385 |
| | v-c | Cluster – analyzed points in terms of groups | 0.158 | 0.182 | 0.038 |
| | v-x | using visual axes to assist in the task | 0.632 | 0.697 | 0.385 |
| | v-s | using a shape feature (valley, shoulder, contour) | 0.158 | 0.121 | 0.038 |
| | v-h | used specific colors (hues) to make decision | 0.316 | 0.242 | 0.308 |

| Category | | | | | | | Role Selectors -> |
|---|---|---|---|---|---|---|---|
| **Strategies** | **Code** | **Description** | Count PSVT-R | Count Pie | Count Scatter | Count Isocontour | **Totals** |
| | s-s | specific – describe a specific strategy that may or may not be discretized that could inform another person in creating his/her own strategy. Strategy is potentially reproducible | 8 | 9 | 9 | 8 | **34** |
| | s-d | discreet steps, the same step repeated | 28 | 14 | 7 | 0 | **49** |
| | s-p | used prop/hand/external aid | 24 | 3 | 1 | 0 | **28** |
| | s-t | skill transference, metaphor usage (mapping) | 3 | 0 | 4 | 2 | **9** |
| | s-m | nonspecific mental visualization (e.g. "imagined it", "visualized it") | 19 | 8 | 18 | 10 | **55** |
| | s-i | using interaction | 0 | 0 | 25 | 42 | **67** |
| | s-o | following an ordered approach (e.g. small to large; faces in sequence) | 0 | 13 | 2 | 2 | **17** |
| | q | mentioned difficulty, confusion | 0 | 0 | 7 | 6 | **13** |
| | s-u | strategy as described is unclear | 6 | 14 | 7 | 7 | **34** |
| | s-e | followed a process of elimination | 4 | 0 | 3 | 0 | **7** |
| | s-a | rapidly alternating between views | 0 | 8 | 0 | 0 | **8** |
| | s-y | Symmetry – discussed symmetry concept (e.g., reflection, rotation, or discussions of symmetry related concepts: handedness, chiral, stereo) | 1 | 4 | 4 | 0 | **9** |
| | s-r | Mirror – mentioned the mirror image relationship of opposite sides. Note that mirror is special case of the symmetry label. | 0 | 0 | 8 | 0 | **8** |
| | | | | | | | |
| **Generated Landmarks** | g-axes | using axes to navigate task (when axes are not present); note in PSVT there were no axes provided | 4 | 0 | 0 | 0 | **4** |
| | g-ref | using generated reference points such as characteristic angles (e.g., 90 deg) or creating groups of angles | 0 | 10 | 0 | 0 | **10** |
| | | | | | | | |
| **Visual Landmarks** | v-u | using a unique component, corner, edge, or face for reference | 18 | 2 | 4 | 0 | **24** |
| | v-z | unspecified mention of size | 0 | 14 | 0 | 0 | **14** |
| | v-r | using area to compare sizes | 0 | 1 | 0 | 0 | **1** |
| | v-a | using angle or arc to compare sizes | 0 | 18 | 0 | 0 | **18** |
| | v-o | Outlier – used outliers/maxima/minima to perform task | 0 | 0 | 14 | 23 | **37** |
| | v-c | Cluster – analyzed points in terms of groups | 0 | 0 | 10 | 0 | **10** |
| | v-x | using visual axes to assist in the task | 0 | 0 | 2 | 45 | **47** |
| | v-s | using a shape feature (valley, shoulder, contour) | 0 | 0 | 7 | 4 | **11** |
| | v-h | used specific colors (hues) to make decision | 0 | 19 | 0 | 7 | **26** |

| % PSVT:R | % Pie | % Scatterplot | % Isocontour | **Mean % CS by task** | **% CS mentioned at least once** |
|---|---|---|---|---|---|
| 1.000 | 1.000 | 1.000 | 1.000 | | **1.000** |
| 0.000 | 0.263 | 0.000 | 0.211 | **0.118** | **0.421** |
| 0.526 | 0.105 | 0.211 | 0.000 | **0.211** | **0.579** |
| 0.263 | 0.000 | 0.000 | 0.000 | **0.066** | **0.263** |
| 0.053 | 0.000 | 0.053 | 0.053 | **0.039** | **0.105** |
| 0.211 | 0.158 | 0.316 | 0.053 | **0.184** | **0.474** |
| 0.000 | 0.000 | 0.368 | 0.474 | **0.211** | **0.579** |
| 0.000 | 0.263 | 0.053 | 0.000 | **0.079** | **0.263** |
| 0.000 | 0.000 | 0.000 | 0.053 | **0.013** | **0.053** |
| 0.053 | 0.211 | 0.105 | 0.158 | **0.132** | **0.316** |
| 0.053 | 0.000 | 0.000 | 0.000 | **0.013** | **0.053** |
| 0.000 | 0.000 | 0.000 | 0.000 | **0.000** | **0.000** |
| 0.000 | 0.000 | 0.000 | 0.000 | **0.000** | **0.000** |
| 0.000 | 0.000 | 0.053 | 0.000 | **0.013** | **0.053** |
| | | | | | |
| 0.000 | 0.000 | 0.000 | 0.000 | **0.000** | **0.000** |
| 0.000 | 0.000 | 0.000 | 0.000 | **0.000** | **0.000** |
| | | | | | |
| 0.158 | 0.053 | 0.053 | 0.000 | **0.066** | **0.211** |
| 0.000 | 0.263 | 0.000 | 0.000 | **0.066** | **0.263** |
| 0.000 | 0.000 | 0.000 | 0.000 | **0.000** | **0.000** |
| 0.000 | 0.263 | 0.000 | 0.000 | **0.066** | **0.263** |
| 0.000 | 0.000 | 0.053 | 0.368 | **0.105** | **0.421** |
| 0.000 | 0.000 | 0.158 | 0.000 | **0.039** | **0.158** |
| 0.000 | 0.000 | 0.105 | 0.632 | **0.184** | **0.632** |
| 0.000 | 0.000 | 0.105 | 0.053 | **0.039** | **0.158** |
| 0.000 | 0.316 | 0.000 | 0.000 | **0.079** | **0.316** |

| 2.000 | 2.000 | 2.000 | 2.000 | | **2.000** |
|---|---|---|---|---|---|
| % PSVT:R | % Pie | % Scatterplot | % Isocontour | **Mean % Chemisty by task** | **% Chemistry mentioned at least once** |
| 0.182 | 0.121 | 0.152 | 0.121 | **0.144** | **0.424** |
| 0.273 | 0.061 | 0.030 | 0.000 | **0.091** | **0.333** |
| 0.212 | 0.030 | 0.000 | 0.000 | **0.061** | **0.212** |
| 0.061 | 0.000 | 0.091 | 0.030 | **0.045** | **0.121** |
| 0.273 | 0.091 | 0.212 | 0.061 | **0.159** | **0.394** |
| 0.000 | 0.000 | 0.242 | 0.697 | **0.235** | **0.758** |
| 0.000 | 0.121 | 0.030 | 0.030 | **0.045** | **0.182** |
| 0.000 | 0.000 | 0.030 | 0.030 | **0.015** | **0.061** |
| 0.091 | 0.152 | 0.121 | 0.030 | **0.098** | **0.273** |
| 0.061 | 0.000 | 0.091 | 0.000 | **0.038** | **0.152** |
| 0.000 | 0.121 | 0.000 | 0.000 | **0.030** | **0.121** |
| 0.030 | 0.030 | 0.121 | 0.000 | **0.045** | **0.182** |
| 0.000 | 0.000 | 0.212 | 0.000 | **0.053** | **0.212** |
| | | | | | |
| 0.121 | 0.000 | 0.000 | 0.000 | **0.030** | **0.121** |
| 0.000 | 0.242 | 0.000 | 0.000 | **0.061** | **0.242** |
| | | | | | |
| 0.333 | 0.030 | 0.091 | 0.000 | **0.114** | **0.364** |
| 0.000 | 0.182 | 0.000 | 0.000 | **0.045** | **0.182** |
| 0.000 | 0.030 | 0.000 | 0.000 | **0.008** | **0.030** |
| 0.000 | 0.303 | 0.000 | 0.000 | **0.076** | **0.303** |
| 0.000 | 0.000 | 0.182 | 0.273 | **0.114** | **0.364** |
| 0.000 | 0.000 | 0.182 | 0.000 | **0.045** | **0.182** |
| 0.000 | 0.000 | 0.000 | 0.697 | **0.174** | **0.697** |
| 0.000 | 0.000 | 0.121 | 0.091 | **0.053** | **0.121** |
| 0.000 | 0.182 | 0.000 | 0.121 | **0.076** | **0.242** |

| 3 | 3 | 3 | 3 | | **3.000** |
|---|---|---|---|---|---|
| % PSVT:R | % Pie | % Scatterplot | % Isocontour | **Mean % Education** | **% Education mentioned at least once** |
| 0.077 | 0.000 | 0.154 | 0.000 | **0.058** | **0.192** |
| 0.346 | 0.385 | 0.077 | 0.000 | **0.202** | **0.615** |
| 0.462 | 0.077 | 0.038 | 0.000 | **0.144** | **0.500** |
| 0.000 | 0.000 | 0.000 | 0.000 | **0.000** | **0.000** |
| 0.231 | 0.077 | 0.192 | 0.269 | **0.192** | **0.423** |
| 0.000 | 0.000 | 0.385 | 0.385 | **0.192** | **0.500** |
| 0.000 | 0.154 | 0.000 | 0.038 | **0.048** | **0.192** |
| 0.000 | 0.000 | 0.231 | 0.154 | **0.096** | **0.269** |
| 0.077 | 0.192 | 0.038 | 0.115 | **0.106** | **0.346** |
| 0.038 | 0.000 | 0.000 | 0.000 | **0.010** | **0.038** |
| 0.000 | 0.154 | 0.000 | 0.000 | **0.038** | **0.154** |
| 0.000 | 0.115 | 0.000 | 0.000 | **0.029** | **0.115** |
| 0.000 | 0.000 | 0.000 | 0.000 | **0.000** | **0.000** |
| | | | | | |
| 0.000 | 0.000 | 0.000 | 0.000 | **0.000** | **0.000** |
| 0.000 | 0.077 | 0.000 | 0.000 | **0.019** | **0.077** |
| | | | | | |
| 0.154 | 0.000 | 0.000 | 0.000 | **0.038** | **0.154** |
| 0.000 | 0.115 | 0.000 | 0.000 | **0.029** | **0.115** |
| 0.000 | 0.000 | 0.000 | 0.000 | **0.000** | **0.000** |
| 0.000 | 0.115 | 0.000 | 0.000 | **0.029** | **0.115** |
| 0.000 | 0.000 | 0.269 | 0.269 | **0.135** | **0.385** |
| 0.000 | 0.000 | 0.038 | 0.000 | **0.010** | **0.038** |
| 0.000 | 0.000 | 0.000 | 0.385 | **0.096** | **0.385** |
| 0.000 | 0.000 | 0.038 | 0.000 | **0.010** | **0.038** |
| 0.000 | 0.269 | 0.000 | 0.115 | **0.096** | **0.308** |

| sessionid | fieldofstudy | Rotation | Code | Pie Chart | Code | 3D Scatterplot | Code | IsoContour | Code |
|---|---|---|---|---|---|---|---|---|---|
| 107899 | 1 | i tried to imagine the rotation/movements needed to achieve the desired 'rotation' -- i then replicated the movement/rotations to each possible choice. | s-d | i tried to ensure that the pie chart had equal pieces, and then compared each piece size | s-d | i tried to rotate the 3d plot to a view that looked similar to the 2d one, imagining myself standing from a position where they would both look equal | s-i,s-m | i tried to relate the 'peaks' in the 3d graph with the circle shapes in the 2d plot | s-s,v-o |
| 120169 | 1 | mapping the rotations in the first image first, then applying it to the real image. Also intuition based on engineering design courses. | s-d,s-t | This was much harder. Different colors beside each other change the perception of the %. I would try to mentally record the relative angle of each slice. | s-m,s-c,v-a | A lot more guessing in this one, a lot of color and shape blending. I would try considering the pattern of increase and decrease for the points and choose the face the repersents the best direction. Then I would consider any outlier points. | ?,v-s,v-o | Base this on the translation of the axis. One problem I found was forgetting is if the contours are in or out the page from the 2d plot | s-u,v-x,q |
| 186136 | 1 | I represented the rotation of the object with the rotation of my fingers to aid in the task. | s-p | I started by comparing smallest slices and then moved to the larger slices in case of difficult examples | s-o | I used the outliers as well as the general shape of the 3D plot to approximate the 2d plot | s-o,v-s | I used the presence of maxima and minima to match the 3d plot with 2d plot | s-s,v-o |
| 215510 | 1 | I would try and focus only on one rotation and see what face I would see in one particular area. So instead of thinking about multiple rotations I would try to narrow down as many options as possible doing this. The questions got particularly difficult at the end. | s-d,v-u | I would look at the smaller slices. It was very difficult to tell differences in larger slices but smaller ones it was possible. | s-s,s-o | I would rotate it a bit to get a feel for the correct angle x,y, or z. Then I would decide which side I was looking from. So a two step proces. | s-i,s-d,v-x | I would align the x and y axis and then see if the contour matched up. | s-i,v-x |
| 246262 | 1 | Identified which faces were facing me initially, and then where they were located after the rotation, and if they changed position on the axis: IE: 90d turn on Z axis, 180d turn on X. I then visualized the presented object with those rotations in my head (or tried too) | s-d,s-m | Compared the arc-size of each colored part of the pie chart. | s-d,v-a,v-h | Visualized the 3D faces in my mind, and tried to determine which face best fit the 2D face given the pattern/direction of the dots. | s-m | Lined the red and blue vectors up with the ones shown in the 2D representation and then compared the topographical map with the 3D model. If peaks and valleys were in the same place, good. If not, or were not represented entirely (IE: peak fully visible in topographical picture but not in 3D), then they did not match. | s-i,v-x,v-o |
| 272439 | 1 | I used my hand as a 3d plane and rotated it the same way and tried to copy that rotation on the new figure. | s-p | Pretty much just eyeballed the size of each slice of the pie. Rotating my head around to see if the slices were the same size. | s-m,v-z | Tried to imagine what it would look like if I could rotate even farther then the figure let me. Looked for large clumps as a "landmark" to base it off of as well. | s-m,v-c,s-i | Same idea with the scatter plot; imagined what it would look like if I could rotate more. Seeing if the tips of the shape matched up with the 2d figure as well. | s-i,s-m,v-o |
| 495443 | 1 | Picked a side, used the palm of my hand to represent that side. Rotated my hand to get to new position, performed same rotation with second set of blocks. | s-p,v-u | Looked at biggest section and saw if colours matched up. Continued that as sizes got smaller. | s-o,v-h,v-z | Rotated and estimated views from missing sides | s-m,s-i | Rotated and matched axes | s-i,v-x |
| | | | | | | | | | |

| | | | | | | | | | |
|---|---|---|---|---|---|---|---|---|---|
| 521767 | 1 | I mentally visualize the rotations necessary to achieve the final result and replicate them in the new piece | s-d | I first see if there is any big discrepancy in the size of each slice. If not, I see if the lines of the big slices are in the same position. If they are, I use them as a base to compare the small slices. If they are not, I try to compare the volume of each slice. | s-o,v-a,v-z | First I see which axis (X, Y or Z) resembles the 2d image the most. After I check if the positive or negative axis fits best. | s-d,v-x | I start by checking which axes are the references of the 2d image, and then I check the position of the highest/lowest peaks to the base of each axis and to the other peaks. | s-s,v-x,v-o |
| 620652 | 1 | mental rotation | s-m | 0 | | 0 | | 0 | |
| 651931 | 1 | doing sidewise rotation, and fixing one side (most of the time the backside) and then compare where the backside is and its current orientation. | s-d | comparing the size | s-u,v-z | This task was a bit unclear. I selected the side I felt I would look at to see the 2D plot | s-u,? | Rotate the axis of the 3D plot to match with 2D orientation, and then compare the contour | s-i,v-x |
| 677187 | 1 | Thought about how it turned each time | s-m | Eye test for each slice | s-u | idk | ? | Didn't realize the axes were provided at first. That made it much easier | v-x |
| 736207 | 1 | Used hand gestures while thinking about turns. When turning, tried to imagine it in one or two steps. Two step turns were done by imagining that the object was made to stand upright on water the bottom face would be, and then rotating it to final position. When in doubt, looked at where the biggest face would end up (e., g, the example here has the square staying at the bottom) | s-d,s-p,v-u | Looked at thinner slices to compare, then looked at colors | s-s,s-o,v-a,v-h | Focused on corner configuration and always turned left-right before up-down | s-i,s-d,v-u | Turned plot such that red-blue formed the bottom square (i.e., the plane the red contour covers fully in the example figure given here) and looked at the purple points to compare | s-s,v-x,v-o |
| 760390 | 1 | calculus | s-u | comparison between the color size | s-s,v-h,v-z | just density of the dots from different perspective | s-u,v-c | dragging the mouse and check from different views | s-i,s-u |
| 794263 | 1 | Using my hand to gesture performing the rotations | s-p | Matching colors, then looking for discrepancies in the angle | s-s,v-h,v-a | Rotating the cube as far as possible in each direction, and then taking my best guess | s-i,s-d | Aligning the red and blue axes in the 3D plot so they matched to isocontour, and then looking at the position of the peaks | s-i,v-x,v-o |
| 799252 | 1 | Visualization and imagination | s-m | comparison | s-u | imagination | s-m | Hovering my mouse and see the bold points | s-u |
| 841530 | 1 | 0 | | 0 | | 0 | | 0 | |
| 866206 | 1 | I tried to mentally "tumble" and "rotate" the example object until it reached the final form, keeping a mental note of the sequence of steps I took. Then I tried to mentally reproduce the sequence of steps on the new object | s-d | I tried to group different colors and see if they still take approximately the same area of the total chart. If the colors happen to not be adjacent anymore, I compared each group individually on both charts. | s-s,v-u,v-h | I tried to think as if the points were droplets of paint and the face was a sheet of paper that pressed against the droplets. | s-t,v-c | I tried imagining standing by one of the 2D axes and looking at the curve as if it was a mountain, then compared to see if the peaks aligned with the 3D contour | s-t,v-s,v-x |
| 906797 | 1 | I flipped the models on 90 degree atomic rotations in my head and performed the same rotation steps on the required model. | s-d | Just tried to see if any piece is slight different. | s-m | tried to visualize from one side, the opposite would have been a mirror so kept that in mind. | s-r,s-m | Had to align the 3d axis with the 2d one which made it easy. | s-i,v-x |
| 987087 | 1 | I first found the sequence of rotations on the first block and then applied those rotations on the second block. After that, I did process of elimination if I was unsure. | s-d,s-e | I compared the category magnitude of each. | s-u | I rotated the graph around to see if I could find the projection. | s-i | I shifted the graph to matches the axes. (Red & Blue Axis) | s-i,v-x |

| | | | | | | | | | |
|---|---|---|---|---|---|---|---|---|---|
| 112441 | 2 | imagine the angle it needs to rotate | s-m | match area of each pie charts | s-u,v-r | just imagine rotating the cube | s-m | match with the axis | v-x |
| 210724 | 2 | Look at two faces and how they would rotate | s-s,v-u | look that the thickness of 2-3 pieces | s-s,v-u | look for patterns in the plot | s-u,v-s | Align the axis to match the two images | s-i,v-x |
| 212834 | 2 | See how top surface rotate | s-s,v-u | compare the size from largest to smallest | s-o | rotate the 3D chart, see which corner fell the most dots | s-i,v-u | 0 | |
| 221034 | 2 | I focused on the long lines and big gaps to identify the rotations | s-u,v-u | I started comparing the pieces in the following order: biggest, smallest, intermediate size. | s-o | I started from identifying the side from which the scattered points could be seen in the required shape (a line, a triangle along certain diagonal, etc). Finally, I tried to match distinctive features such as isolated points. | s-s,v-s,v-u | Started from matching the axis and checking for the correct location of the highest points. Later I would check for distinctive features such as halves and incomplete hills. | s-i,v-x,v-o,v-s |
| 240265 | 2 | flipping the block. | s-u | size change | s-u,v-z | visualizing the dots fall on to a surface | s-m | rotating the graph and superimposing. | s-i |
| 243972 | 2 | Pick a side that really stands out (usually the two bars) and figure out the way of rotation using that side. Then operate that way of rotation on the other object. | s-s,v-u | Visually estimate the size of each colour | s-s,v-z,v-h | Move around until a side looks close to the given plot or the symmetrical counterpart of it. Decide a phase from there | s-y,s-i | Move around so that the axes on the 3D plot matches those of the 2D plot. Then find the most prominent peaks on the 3D plot and compare them. | s-i,v-x.v-o |
| 259535 | 2 | I didn't really have a strategy for the simple shapes (ie, shapes with right angles only) undergoing single-axis rotations - my brain just did it. However, when there was a complicated shape (ie, contained 45 degree angles or cylinders) or when rotating along multiple axes, I simplified the problem by picking one face and rotating that instead of the whole shape. I always broke it down into stepwise individual rotations. Once my strategy worked on the example shape, I repeated it once or twice on the test shape. I also simulated the rotation with my hands for some of the trickier ones, it helped me to focus/concentrate. | g-axes,s-d,s-p,s-s | These were hard! I roughly compared the ratio of the arc lengths between some of the segments, in my brain, until I found a pair that didn't match. If they all seemed to match, I tried looking at the angles for a bit longer before clicking 'yes'. I also tried to compare the segment angles to more recognizable ones (90 degrees, 45 degrees or 180 degrees) when possible, to make for easier comparison between pie charts (this worked when adding segments together, as well). It was harder to gauge a change in large-angle segments, or when the segments were all similar in size. A few times, I used my fingers to guestimate an arc length and overlay it on the neighboring shape (hope this isn't considered cheating - no rulers/protractors!) | v-a,g-ref,s-p | When the data was grouped in distinct areas, I could sometimes recreate a similar reflection of the data and then knew it was viewed from the other side. When the data was more evenly dispersed, it was more difficult. In these cases, I tried to look for outlying data points near the edges of the cube, especially ones that were closer to one side than the other, and use these to orient myself. It was often more helpful to look at outliers than the bulk of the data points. Sometimes if these were not available, I looked for 2-3 closely spaced/colinear points in the 2D image and tried to locate suitable candidates in the 3D cube while rotating the image. In one case where the points seemed more discrete/quantized/colinear from one or two specific angles, I tried to emphasize the outlier points to avoid being tricked by an optical illusion (but maybe I got this one wrong, who knows!) | s-y,s-r,v-o,v-c,s-i | First I rotated the 3D shape to align the red/blue axes with the 2D image as well as possible. If the shapes roughly aligned, I then rotated the 3D image upward so the blue axis bisected the data, and compared the spacing between 3D peaks (and/or the side slope) with the 2D plot. In some cases, I then rotated 90 degrees so the red axis bisected the data (from the front) and did the same. For peaks located near an axis, I looked closely at the rotated 3D plot to judge whether the feature had been cut off before or after a local maximum, and if this matched with the 2D plot. A few times I also rotated further (putting the blue/red axis at the back) to look at peaks far from an axis in the same way. In a few cases, I compared the purple intensity of the 2D and 3D plots to see if the order of the peak heights was the same in both. I also looked for the number of peaks in the contour plot and compared it to the number of 'resolvable' peaks in the 3D plot (there was one shape which had two overlapping peaks that weren't quite resolved, in my mind). If I found no issues, I clicked 'yes'. | s-s,s-i,v-x,v-o |
| 306274 | 2 | Just rotate it in my mind | s-m | Visual comparison | s-u | Imagining different perspectives | s-m | Just rotating | s-i |

| | | | | | | | | | |
|---|---|---|---|---|---|---|---|---|---|
| 332599 | 2 | Determined which rotations were done to the first image (flip horizontally, rotate 90 degrees left etc) and then apply to the second object. | s-d | Some charts were quite obviously different or the same, but on those that were tricky, measuring the width / angle of slices on the chart confirmed if they were different fairly quickly. | v-a | Look at which side of the 2D face the dots are on, and see which face of the cube corresponds. | s-u | Lining up the red/ blue axes so the 3D and 2D could easily be compared. | s-i,v-x |
| 364390 | 2 | mental rotation of the object, used hands as well | s-p,s-m | none, it was easy | s-m | tried to imagine which face of cube was closest to the darker (closer) dots | s-m,v-c | mentally rotated axes in head | s-m,v-x |
| 388991 | 2 | Finding out in which ways the first images were rotated, then visualizing how the shape would look if rotated the same ways (i.e. rotated down then left, or upside down). | s-d | Visualizing measuring widths of the smallest pie slices first, then looking at the biggest slices to finally compare | s-o | Rotating the block to see the most similar spots to the image. | s-i | Rotating the 3D image so that the axes matched, then looking where "apexes" are in the 3D image vs the 2D image | s-i,v-x,v-o |
| 389400 | 2 | Rotated the example object and the rotated the object in question (looked at the vertices of the example object and applied it to the question object). Also if there were two rotations I did one rotation with the example object and the question object, and then did the second rotation with them. | s-s,s-d,v-u | Looked for any differences in sizes of the slices based on how much space each slice took up of the outer diameter of the circle. | v-a | I was able to picture where the dots were positioned and more dense when looking at it from each face. Also looking for outlier dots on the plot and where it would be when looking from each face was also helpful. | s-u,v-o,v-c | Moved the axis so that they were lined up the same. Looked at where the peaks were located and then looked at where the highest intensity peak was. | s-i,v-x,v-o |
| 418479 | 2 | Visualizing the object and imitating the rotation with my hand | s-p | 0 | | Looking at lone points that are in a specific corner of the plot | s-o,v-u | 0 | |
| 581241 | 2 | focus on one side | v-u,s-u | compare each pieces separately | s-d,s-u | find the opposite side | s-r | rotate the axis to the right position | s-i,v-x |
| 585666 | 2 | "tumbling", i.e. rotating the shape by 90 degrees along different axes. | s-d,g-axes | 1st step: comparison, color by color, between the left and right sides<br>2nd step: (occassionnally) comparing two neighbouring colors to see if their ratio appears to remain the same.<br>3rd step: Looking specifically at pies close to 80 degrees and trying to compare how much they differ from a straight angle. | s-a,v-h,g-ref,v-a | 1) Spotting the highest density of dots<br>2) Making sure that this high density of dots appears in the right quadrant of the face I am looking through.<br>3) Making sure that the dots "far away" from the high density appear in the right quadrant too. | s-s,v-c,v-s | 1) Orienting the red/blue axes<br>2) Making sure that the blue peaks track<br>3) Making sure that the orange peaks track<br>4) Making sure that there is no extra peak. | s-i,v-x,v-o,v-h,v-s |
| 590156 | 2 | Rotate the object step by step (starting with a rotation along the first axis and afterwards on the second axis) | g-axes,s-d | Try to find patterns (like two fields occupying half of the circle) | s-s,g-ref | Use the big amount of dots to decide wether it is top/bottom, front/back or left/right. Use the postion of isolated dots to decide on the exact view. | s-r,v-o,v-c | Regard the 3D plot along the two axis and compare the position of the peaks. | s-i,v-x,v-o |
| 614589 | 2 | Used my hand to figure out rotations of L shapes | s-p,v-u | Glanced back and forth between the same color on the two different charts to decide if they were the same size | s-a,v-h,v-z | Process of elimination of the sides that I could view in the 3D plot | s-e,s-i | Aligned the axis of the 3D plot with the 2D plot (started doing after the first 4) | s-i,v-x |

| | | | | | | | | | |
|---|---|---|---|---|---|---|---|---|---|
| 620339 | 2 | Visualized picking up and rotating the object as if it was in front of me then doing the same with each test object. Interestingly sometimes the shapes would "fall flat" and it would be very hard to picture them as 3D objects | s-m,s-s | Rapidly looked between the charts to look for differences in size between each segment | s-a,v-z | Pictured what it would look like for an observer of the sides I wan't able to view from | s-m | Matched the axes then compared peaks (number, height, placement if viewed from above) | s-i,s-s,v-x,v-o |
| 642006 | 2 | Looked at anchor faces such as where the bottom or top ended up and attempted to have that reflected on the 3d rotated shape. | v-u,s-m | Looked at each colour individually and checked that they were the same size on each. | v-h,v-z | Mostly a guess attempted to line up and rule faces out. | s-e,? | lined up the xy plane with the orientation on the left-hand side. | s-i,v-x |
| 647517 | 2 | Thinking through the rotation steps one at a time and trying to visualize the result of each step. | s-d | Comparing individual sections, looking at benchmarks like 1/2 or 1/4 if applicable. | g-ref,s-s | Identifying key features and their placement (either large groups of dots or isolated dots), thinking of the mirror image to visualize the back square. | s-s,s-r,v-c,v-o | Orienting the 3-D version so that it lined up with the 2-D version before comparing. | s-i |
| 651941 | 2 | The simple ones I just rotated mentally. For the more challenging shapes I compared which faces moved where. For example, here the back-right face becomes the front right face. From there, process of elimination if the answer wasn't readily apparent. | s-m,v-u,s-e | Looked at the angles made by different coloured pieces of pie, and the combined angles when similar colours were grouped together in both pies. | g-ref,v-h,v-a | Tried to visualize myself looking through a particular face of the box | s-m | Rotated to match the correct axes, and checked if things lined up. | s-i,v-x |
| 681524 | 2 | Imagined I was Tony Stark in the first Iron Man movie, in the scene where he is in his workshop, and he has a hologram where he can rotate a 3D design object with his hand. | s-p | I looked at angles, and tried to ignore colors. | v-a | Imagine I was walking around a fish tank, and trying to see which side would give me the 2D projection of the data. | s-t,s-m | Focused on matching the axes, and then it was just like reading a topographical map. | s-i,v-x,s-t |
| 685932 | 2 | 0 | | 0 | | 0 | | 0 | |
| 688752 | 2 | Visualizing rotations by moving and rotating hands to move image in head. | s-p | Fast comparison between individual slices. Rotating slices in head to match other chart and compare angles. | s-a,s-m,v-a,s-y | Move 3D chart and visualization of that side | s-i | Reorient 3D plot such that axis origin matches the one seen in 2D plot. Then compare peak locations to see if close to contour plot. If similar then looking to see if gradation matches 2D contours. | s-s,s-i,v-x,v-o,v-h |
| 714014 | 2 | imagine it | s-m | just stare at it | s-m | try to see it from that side. flip the image in your head | s-i,s-r | match the axis so that its just a basic compariison | v-x |
| 735535 | 2 | Rotating in my head. In practice, I would build a model to do the necessary rotations for molecules | s-t,s-m | Comparing to 1/2 or 1/4 of a circle. The instructions were too vague for this task. | g-ref | The instructions were too vague for this task. There is a handedness assumed for the data, that I could not figure out. | s-t,q | Rotating the 3D plot | s-i |
| 762315 | 2 | Many of these problems feature problems with the chirality of the answers - you flipped some of them! Several have no correct answer. Learn stereochemistry! | s-y,s-t | 0 | | Your interface doesn't allow complete rotation; and there are redundant answers. | | Your interface doesn't allow complete rotation. | |
| 774440 | 2 | | | compare the sectors to the right angle (>90, <90) and between each other | g-ref,v-a | find outliers, find direction (two faces), find the right "chirality" | s-s,s-r,s-t,s-y | align axes, compare | s-i,v-x |
| 856854 | 2 | Rotation axes | g-axes | Compare individual wedges | s-d | Imagine view from each face | s-d | Imagine view from red-blue plane | s-m |

| | | | | | | | | | |
|---|---|---|---|---|---|---|---|---|---|
| 896485 | 2 | I would visualize the movement step by step. I try to do one rotation, visualize the change, and do it again. I also tried following 1 characteristic face in cases where the shape was very complex. | s-d,v-u | I tried looking at the angles in some cases, although it was really only helpful for larger slices. | s-o,v-a | This one was a little tougher, but I eliminated sides based on the projection. Then I tried to line up unique points (like an isolated dot). | s-e,v-o | I lined up the x and y axis and saw if it matched. I did worry half way through if I missed something in the instructions though! | s-s,v-x,q |
| 912301 | 2 | Think about what the shape looks like at every rotations | s-m,s-e | Sizes relative to each other | s-u,v-z | How the 3D plots will flatten if looked at from one side | s-u | The darker coloured circles are greater heights/depths | s-u,v-h |
| 947555 | 2 | I would look for landmarks, and then break the rotation down into 90 degree segments, then choose a landmark on the second shape, and pull it through the same rotations. | s-d,v-u | I looked for individual segments that form a right angle or a 180 degree angle, or slight deviations therefrom, and also compared the relative size of individual segments. | g-ref,v-a | I looked at the general shape of the data, as well as the relative position of relative outliers from the 2D plot, and tried to find a match to this shape or its mirror image in the 3D plot and its rotations. | s-s,v-s,v-o,s-r,s-y | First aligned the axes, then checked to see if the shape matched. | s-i,v-x,v-s |
| 953397 | 2 | I tried to use my hands to imagine the rotation of the first object to mimic the rotation of the second object | s-p | I visually compared the different individual colours to each other instead of looking at the whole pie chart as one. I felt like I was able to notice more differences that way | v-h | I rotated the 3D box till I thought I could see what was represented in the 2D, this one was hardest for me | s-i,? | This one I matched up the axis and then tried to figure out where the high points (blue contours) would go and decide based off that. Then I would double check with the low orange regions. I would match the location and the intensity of colour | s-i,s-o,v-x,v-h |
| 129382 | 3 | 0 | | 0 | | 0 | | 0 | |
| 133269 | 3 | Imagined holding the object in my hand | s-p | compare each colour one at a time | s-d,v-h | I wasn't sure about this one, as you can get the same view from either side, just rotated, so it seemed a 50% chance each time. | q,s-i | Aligned the axis to same direction and match high points to location | s-i,v-o,v-x |
| 137930 | 3 | Picturing how a specific side needs to rotate in order to get to the final position. Sometimes working backwards from the options to see if there were any that could not be the original shape or it's rotation. | s-e,s-s,v-u | Checking first to see if any colour is easily identifiable as different, then going colour by colour to see if there were minute differences visible. Finally, comparing groupings of colours to see if they match. | s-d,v-h,g-ref | Trying to see where the outliers were and figuring out where they would be visible from each side. | s-s,v-o | Rotating the 3D view so the blue and red axis were the same as the 2D view. Then checking on the position of the various peaks and valleys as compared to 0,0. | s-i,v-o,v-x |
| 185465 | 3 | visual step by step rotation | s-d | colour then size comparisons | s-d,v-h,v-z | rotating the cube to see the best fit | s-i | none | |
| 224364 | 3 | I tried to imagine the shapes rotating in my mind and sometimes I tried pretending I was holding that shape in my hand and rotating it. I also drew some pictures. | s-m,s-p | I examined each sector to see if each coloured sector looked the same size as its corresponding sector. | s-d,v-h | This one was really hard. I tried to look at the scatterplot from different angles in my mind. | q,s-m | I mainly looked at the way the colours dissolved in the 2D graph vs the 3D graph | s-u,v-h |
| 309678 | 3 | Go through steps I would take to make the model match (i.e. turn over to the right, then forward) and try to do the same for the question. | s-d | Compare colour for colour and the one it's beside | s-d,v-h | Try to look to key outliers | s-s,v-o | Look at highest peak | s-m,v-o |

| | | | | | | | | | |
|---|---|---|---|---|---|---|---|---|---|
| 400716 | 3 | I identified one side of the figure and then its location on the rotated image and matched that with the options. I also used my hands to visualize rotating the image to imagine rotating the original and then doing the same with the options. For the rotations that were multi-step, I would try visualize the in-between step(s). Identifying which face the figure was "sitting on" also helped. | v-u,s-s,s-p,s-d | I used my finger and thumb to try and identify angles and size to compare. I also tried to use fractions to identify which colours made up easy fractions like quarters, halves, and thirds to see if they combined to make the same fractions on the image. I'd line up my hand to identify angles and try to see if it matched the other image if there wasn't a rotation of the slices. | s-p,g-ref,s-y | I would identify main shapes in the dots (like a larger blob, smaller blob) and what position the cube would be in to see the dots in that way. I would try visualize looking through the top or side of the cube and identifying where the dots would congregate from that perspective. | v-c,s-d,s-m | I rotated the image so the axes would line up and look for height and corresponding locations on the 3D image. I was looking for general location and relative height of each of the points and I mainly focused on the purple rather than the orange. | s-i,v-x,v-o,s-h |
| 412490 | 3 | Physically moving my hand to imitate the changes to the blocks | s-p | Looking back and forth repeatedly from one chart to the other. | s-a | Moving the 3d cube a lot | s-i | Checking the position of the axes, then the placement of the peaks, then the placement of the valleys | s-i,s-o,v-x,v-o |
| 457768 | 3 | movement from top to bottom placement from side to side | s-u | size of each slice | | no clue | q,v-o | no clue | q |
| 487261 | 3 | Used the mouse to pretend to rotate the blocks | s-p | Compared each colour | s-d,v-h | Rotated the cube | s-i | Rotated the grab to try and match the images | s-i,s-m |
| 487731 | 3 | Describe the moves, then try to do the same with the shape. | s-d | Compare sizes of the slices | s-u,v-z | Highlight and see which looks most like it. | s-i | Orient with the axes. | s-i,v-x |
| 551790 | 3 | visualization of rotations, rotated a deck of cards to help compare physical rotation | s-d,s-p | focus on the smallest colour slice | s-o | purely attempted a best guess | q | purely attempted a best guessed | q |
| 586515 | 3 | I thought of this as a Rubik's cube. I made the motions with my hands of how I would rotate the objects and kept using the same physical motions to help me figure out the answer. | s-p,s-d | my eyes darted back and forth for each color pair and did a rough comparison. sometimes, when the colors appeared in the same order, I tried to visualize a clock-wise rotation of the left pie chart to see if it would match the right one. | s-a,s-y | I looked for key features in the 2d version, such as a large grouping in the lower left corner or a long trail along the top edge. I rotated the cube as much as I could and imagined how the dots would line up if I could fully rotate the cube without restriction. | s-s,v-s,v-o,s-i | I rotated the 3d model until the red axis and blue axis matched the orientation of the 2d representation. from there, I looked at the blue peaks on the 3d version and tried to see if they roughly matched the blue circles on the 2d version. | s-i,v-x,v-o,v-h |
| 589143 | 3 | Tried to focus on visualizing where one of the sides (faces?) rotated (back to top; front to bottom, etc) or visualized the solid in my hand and manually rotated it and then tried to do the same for the second set. | s-d,v-u,s-p | Focused on size of the angles. | s-u,v-a | Zero confidence in what I was doing here. | q,v-o | Zero confidence in what I was doing here. | q |
| 603798 | 3 | mentally rotating (use my hand as a guide) | s-p,s-m | side by side comparison | s-d,s-a | visualization | s-m | visualizing | s-m |
| 665822 | 3 | I used my hands to rotate and imagined the answer before I looked at answers. | s-p | looked at biggest and smallest pieces that did not match | s-o,s-u | looked at different views by turning the cube | s-i | This was the hardest one, I could not visualize, very confusing | q |
| 703754 | 3 | Utilized 3D shape manipulatives. | s-u | None. | | Drawing on paper. | s-p | Visualized. | s-m |
| 764411 | 3 | Thinking about what edge of the sample shape would now be in the front. | s-m,v-u | Looking at the angles made in the centre | s-u,v-a | rotating the 3D representation as much as I could | s-i | Looking where the blue/red axis met | s-u,v-x |
| 803014 | 3 | 0 | | 0 | | 0 | | 0 | |
| 810153 | 3 | two step rotation | s-d | only paying attention to the biggest part | s-o,s-u | totally lost, trying to locate outliers | q,v-o | intersection along the exes | s-u,v-x |
| 827935 | 3 | I tried to imagine the shape being rotated | s-m | compared the colours and tried to be as precise as possible in terms of size | s-d,v-h,v-z | imagined what the view would be from each particular side of the net | s-d | Found this most difficult. tried to envision how it would look and match the colours with the net and amount of circles | ?,s-m,v-h |

| | | | | | | | | | |
|---|---|---|---|---|---|---|---|---|---|
| 843435 | 3 | flipping the image in my head and using my hands | s-m,s-p | looking at each section on it's own and comparing it to the other circle | s-d,s-m | Looking to see if the dots looked like they were in the same space | s-u | 0 | |
| 851243 | 3 | mental visualization | s-m | mental visualization | s-m | mental visualization | s-m | mental visualization | s-m |
| 931997 | 3 | 0 | | 0 | | Rotating the 3D plot | s-i | Rotating the 3D graph | s-i |
| 949909 | 3 | I gestured as though I was holding and rotating the blocks with my hands. | s-p | Sometimes I used my fingers to compare the widest parts of each slice. Either the differences were so slight that I couldn't tell, or there were many pairs that showed the same data. Other times, I imagined rotating the angle of the largest slice to see if it matched the angle in the reference chart. | s-o,s-p,s-y | Rotated the cube on screen, and then rotated the rest mentally. | s-i,s-m | Rotated the graph on screen to match the orientation of both blue axes, then mentally rotated the graph further as necessary to match the reference graph. | s-i,v-x,s-m |
| 999085 | 3 | Figuring out the steps (1/4 turn clockwise on Z, then 1/2 turn CCW on X...) then applying to the model | s-d | Looking at the part of the circumference that each section made up. Flicking quickly between the two diagrams. | s-d,v-a,s-a | Looking and matching up the outliers was helpful for some that could potentially be through multiple sides. | s-s,v-o | Matching the XY axis up then looking at the peaks. Although some seemed close but just "cut off". | s-i,v-o,v-x |
