# Supplementary material for: Professional Differences: A Comparative Study of Visualization Task Performance and Spatial Ability Across Disciplines
Source: arXiv:2108.02333 ancillary file (2021-08-05)
Supplement: Supplementary file 3 [file Quantitative_Analysis_CIs.pdf]

Professional Differences: A Comparative Study of Visualization Task Performance and Spatial Ability Across Disciplines

IEEE VIS 2021

Kyle Hall, Anthony Kouroupis, Anastasia Bezerianos, Danielle Albers Szafir, and Christopher Collins

# Detailed CI reporting for Spatial Abilities (H1) and the three Visualizations (H3).

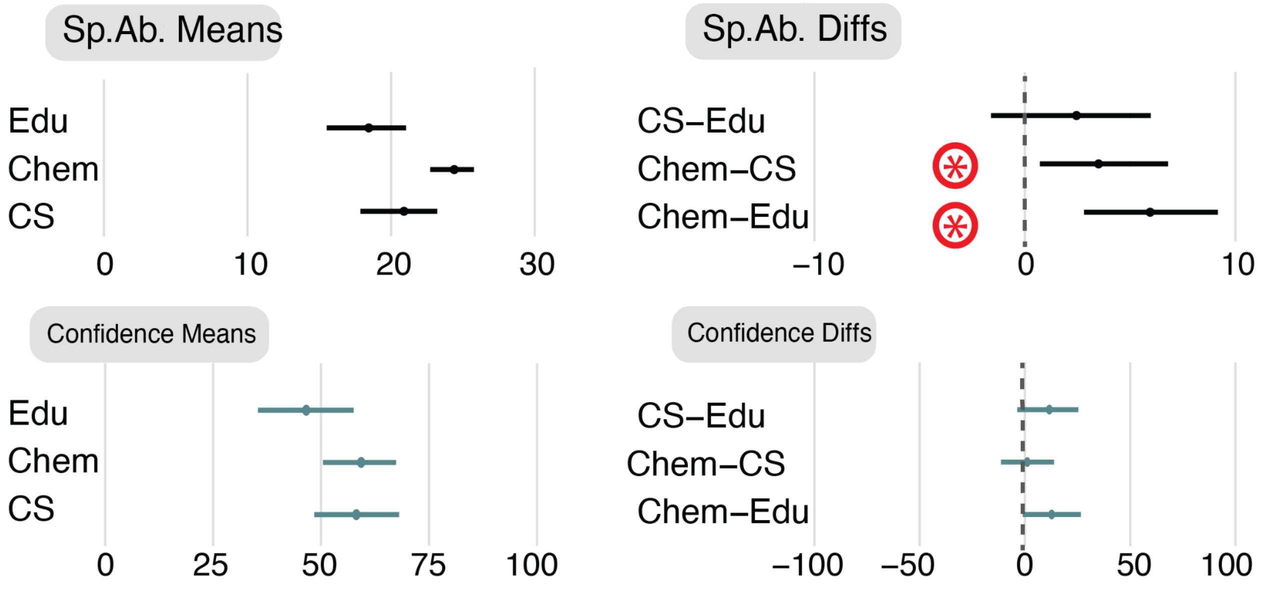


Fig. 5-extended. *H1*:**Spatial Abilities** per Discipline, with the CI of means (left) and of mean differences (right). In the mean differences plot (right) CIs that are tighter and further away from 0 provide stronger evidence of dif-ferences. On the bottom, CIs of means and differences in Confidence for the spatial ability tasks. Red stars indicate evidence of differences between disciplines. Error bars represent 95% Bootstrap confidence intervals (CIs).

Table 1. Detailed CIs for the Spatial Abilities Task.

| | | Means | | Differences |
|---|---|---|---|---|
| Spatial Abilities (out of 30) | Edu<br>Chem<br>CS | 18.44 [15.51; 21.03]<br>24.39 [22.72; 25.75]<br>20.89 [17.86; 23.21] | CS-Edu<br>Chem-CS<br>Chem-Edu | 2.45 [-1.60; 5.97]<br>3.49 [0.71; 6.80] *<br>5.94 [2.80; 9.16] * |
| Confidence (%) | Edu<br>Chem<br>CS | 46.55 [35.38; 57.51]<br>59.27 [50.46; 67.37]<br>58.15 [48.42; 68.05] | CS-Edu<br>Chem-CS<br>Chem-Edu | 11.60 [-3.65; 25.35]<br>1.11 [-11.39; 13.78]<br>12.71 [ -0.99; 26.54] |

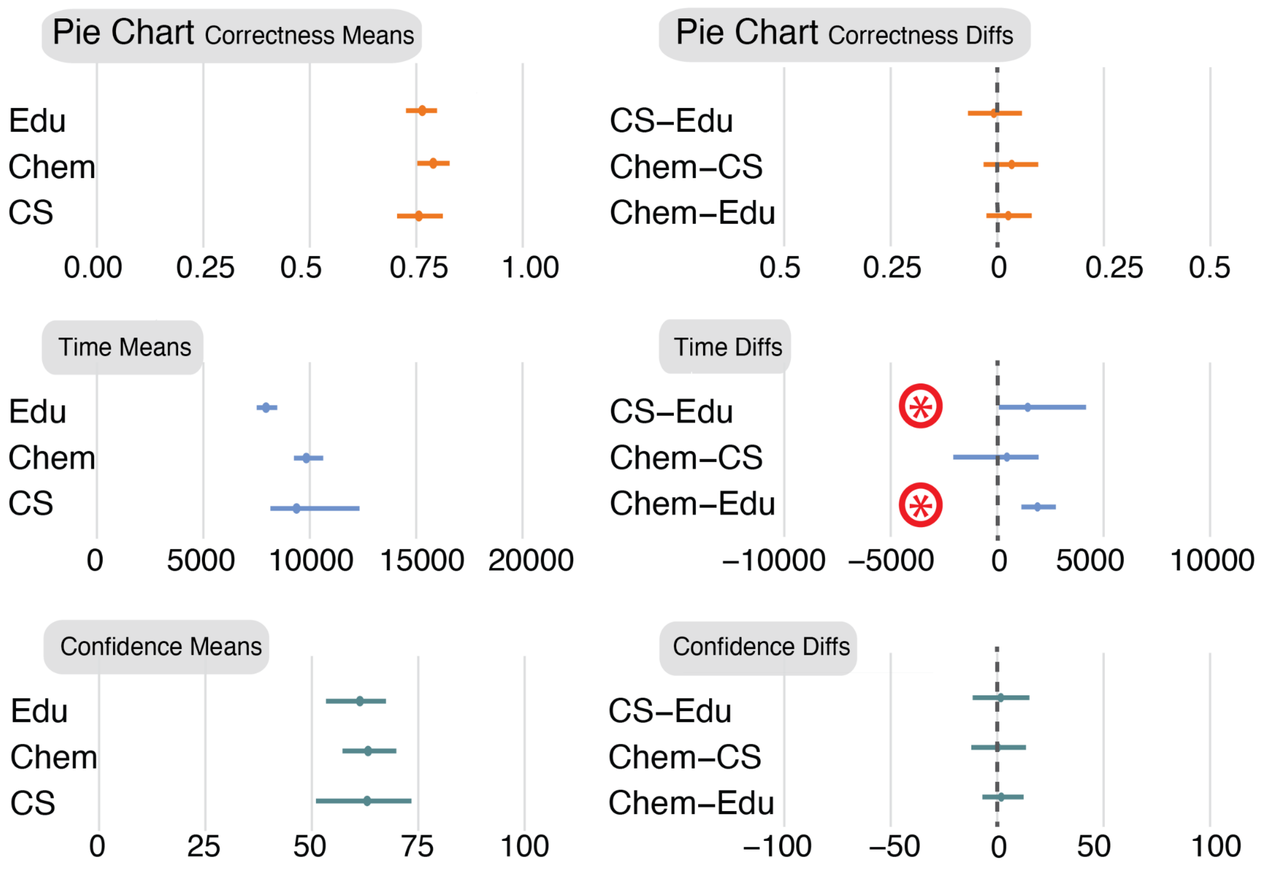


Fig. 7-extended. *H3*-**Pie Chart** performance means (on the left) and mean differences (on the right), for Correctness, Time and Confidence. Red stars indicate evidence of differences between disciplines. Error bars represent 95% Bootstrap confidence intervals (CIs).

Table 2. Detailed CIs for the Pie-Chart Task.

| **Pie-Chart** | | Means | | Differences |
|---|---|---|---|---|
| Correctness Rate (0-1) | Edu<br>Chem<br>CS | 0.76 [0.72; 0.79]<br>0.79 [0.75; 0.82]<br>0.75 [0.70; 0.81] | CS-Edu<br>Chem-CS<br>Chem-Edu | -0.00 [-0.06; 0.05]<br>0.03 [-0.03; 0.09]<br>0.02 [-0.02; 0.08] |
| Time (msec) | Edu<br>Chem<br>CS | 7942.44 [7504.36; 8468.50]<br>9835.94 [9261.10; 10629.18]<br>9378.19 [8151.52; 12337.93] | CS-Edu<br>Chem-CS<br>Chem-Edu | 1435.74 [78.73; 4172.51] *<br>457.75 [-2065.10; 1945.59]<br>1893.50 [1140.73; 2753.37] * |
| Confidence (%) | Edu<br>Chem<br>CS | 61.29 [53.33; 67.40]<br>63.21 [57.21; 69.84]<br>63 [51 ; 73.36] | CS-Edu<br>Chem-CS<br>Chem-Edu | 1.70 [-11.49; 15.14]<br>0.21 [-12.08; 13.49]<br>1.91 [-6.88; 12.35] |

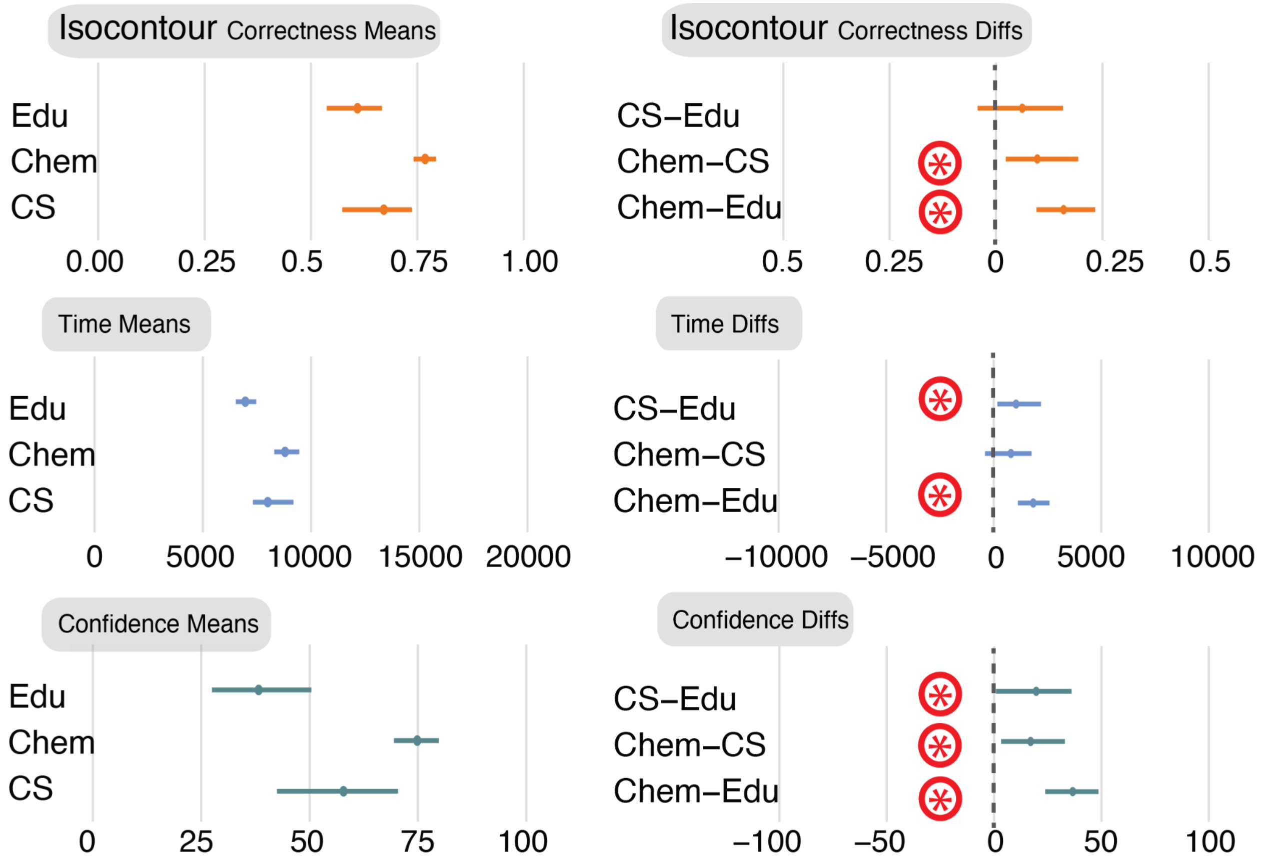


Fig. 8-extended. *H3*-**Isocontour** performance means (on the left) and mean differences (on the right), for Correctness, Time and Confidence. Red stars indicate evidence of differences between disciplines. Error bars represent 95% Bootstrap confidence intervals (CIs).

Table 3. Detailed CIs for the Isocontrour Task.

| **Isocontour** | | Means | | Differences |
|---|---|---|---|---|
| Correctness Rate (0-1) | Edu<br>Chem<br>CS | 0.60 [0.53; 0.66]<br>0.76 [0.74; 0.79]<br>0.67 [0.57; 0.73] | CS-Edu<br>Chem-CS<br>Chem-Edu | 0.06 [-0.04; 0.15]<br>0.09 [0.02; 0.19] *<br>0.15 [0.09; 0.23] * |
| Time (msec) | Edu<br>Chem<br>CS | 6960.42 [6526.14; 7463.66]<br>8796.04 [8298.55; 9455.12]<br>7997.05 [7308.38; 9182.33] | CS-Edu<br>Chem-CS<br>Chem-Edu | 1036.62 [168.43; 2196.26] *<br>798.99 [-405.71; 1755.28]<br>1835.61 [1126.08; 2588.30] * |
| Confidence (%) | Edu<br>Chem<br>CS | 38.25 [27.48; 50.38]<br>74.84 [69.48; 79.83]<br>57.84 [42.47; 70.36] | CS-Edu<br>Chem-CS<br>Chem-Edu | 19.58 [0.86; 36.05] *<br>17.00 [3.25; 32.94] *<br>36.58 [23.80; 48.52] * |

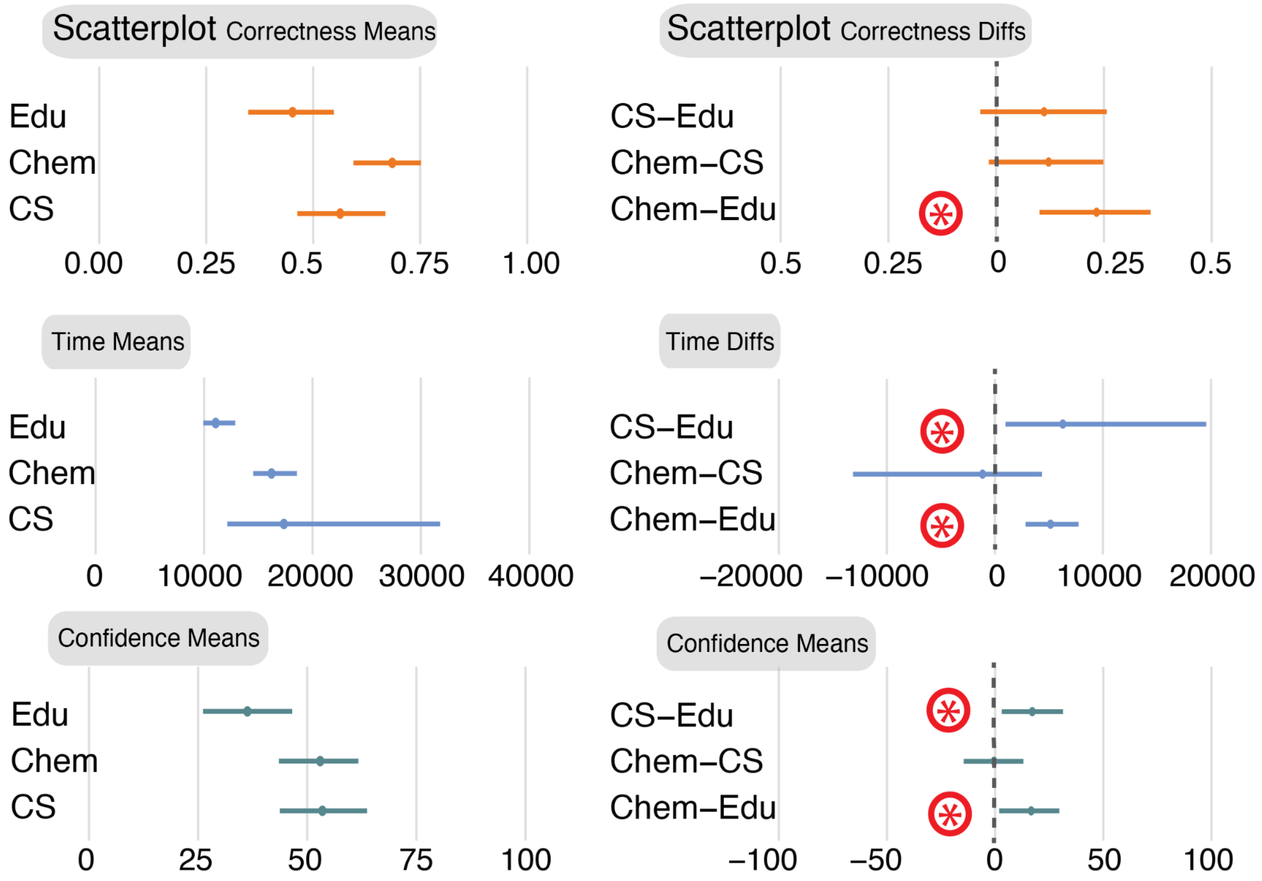


Fig. 9-extended. *H3*-**Scatterplot** performance means (on the left) and mean differences (on the right), for Correctness, Time and Confidence. Red stars indicate evidence of differences between disciplines. Error bars represent 95% Bootstrap confidence intervals (CIs).

Table 4. Detailed CIs for the Scatterplot Task.

| **Scatterplot** | | Means | | Differences |
|---|---|---|---|---|
| Correctness Rate (0-1) | Edu<br>Chem<br>CS | 0.45 [0.34; 0.54]<br>0.68 [0.59; 0.75]<br>0.56 [0.46; 0.66] | CS-Edu<br>Chem-CS<br>Chem-Edu | 0.11 [-0.03; 0.25]<br>0.12 [-0.01; 0.24]<br>0.23 [0.10; 0.35] * |
| Time (msec) | Edu<br>Chem<br>CS | 11072.25 [9927.54; 12867.92]<br>16216.30 [14529.19; 18555.82]<br>17358.73 [12148.42; 31760.52] | CS-Edu<br>Chem-CS<br>Chem-Edu | 6286.47 [978.11; 19553.39]*<br>-1142.43 [ -13126.48; 4344.16]<br>5144.04 [2836.70; 7748.45]* |
| Confidence (%) | Edu<br>Che<br>CS | 36.29 [26.14; 46.56]<br>52.96 [43.52; 61.70]<br>53.47 [43.73; 63.69] | CS-Edu<br>Chem-CS<br>Chem-Edu | 17.17 [3.07; 31.37] *<br>-0.50 [-14.52; 13.03]<br>16.67 [1.88; 29.67] * |
