# Supplementary material for: Professional Differences: A Comparative Study of Visualization Task Performance and Spatial Ability Across Disciplines
Source: arXiv:2108.02333 ancillary file (2021-08-05)
Supplement: Supplementary file 4 [file Study_Sequence_Full.pdf]

# Professional Differences: A Comparative Study of Visualization Task Performance and Spatial Ability Across Disciplines

## Study Design Supplement

IEEE VIS 2021

Kyle Hall, Anthony Kouroupis, Anastasia Bezerianos, Danielle Albers Szafir, and Christopher Collins

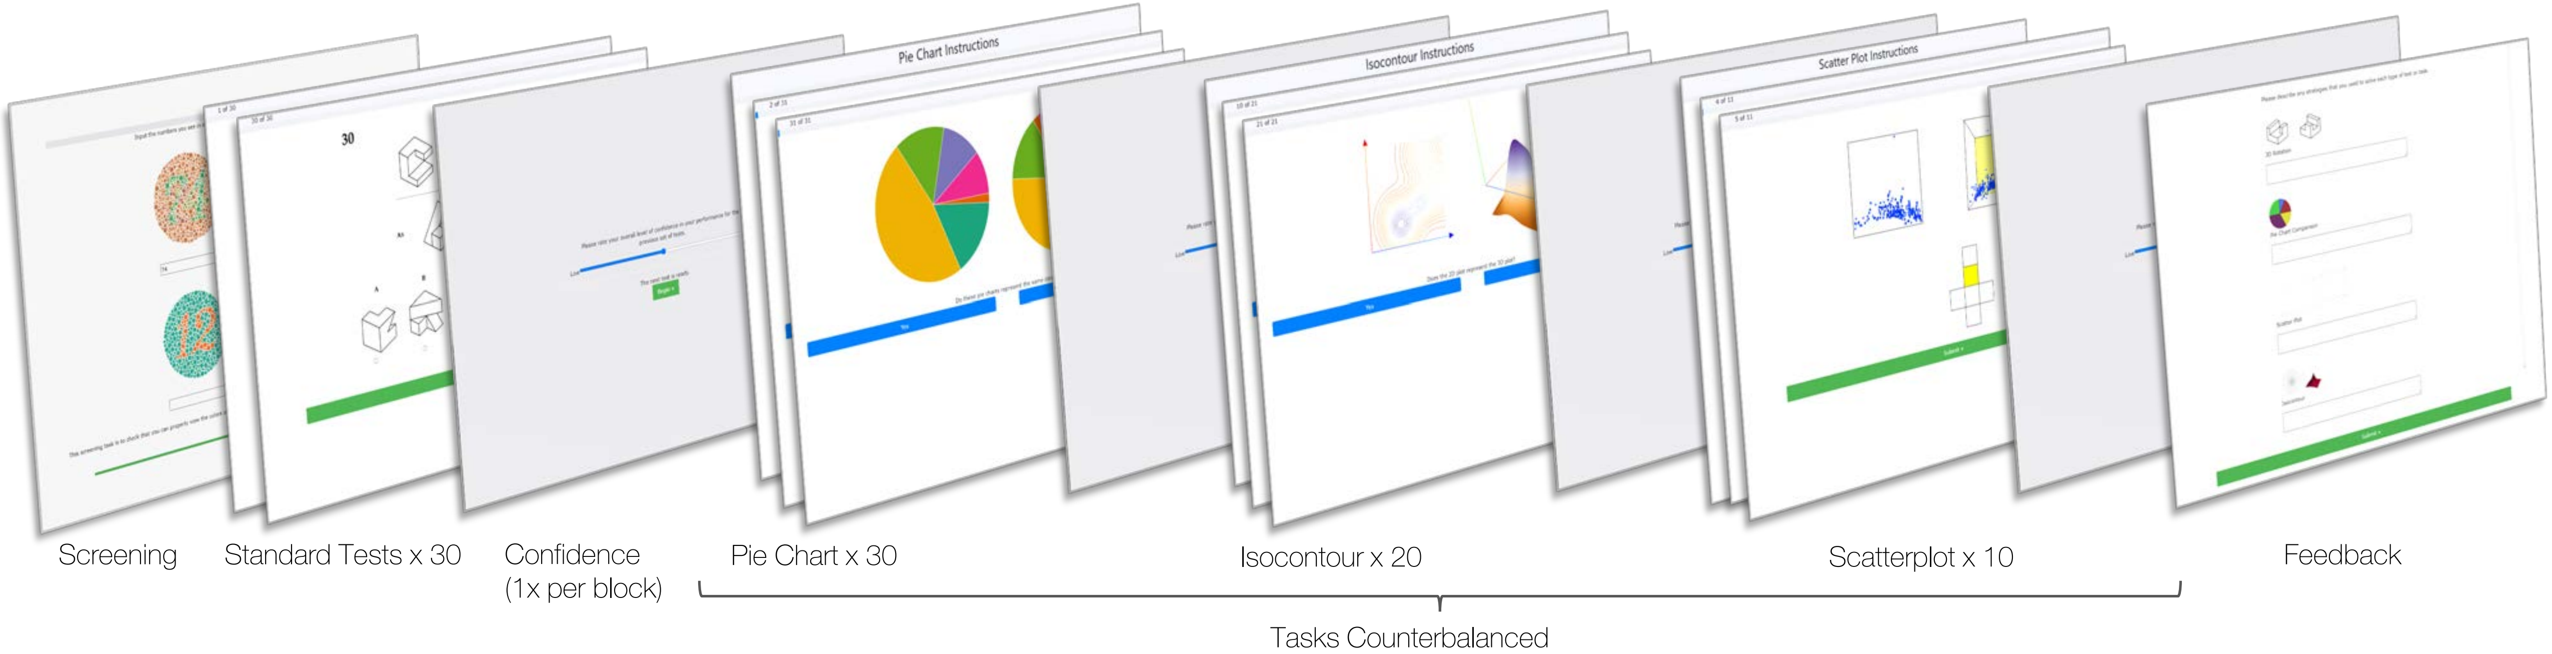

Pie Chart Instructions
Isocontour Instructions
Scatter Plot Instructions
Screening
Standard Tests x 30
Confidence
(1x per block)
Pie Chart x 30
Isocontour x 20
Scatterplot x 10
Feedback
Tasks Counterbalanced

# Screening

Input the numbers you see in each circle in the corresponding textbox, then click submit

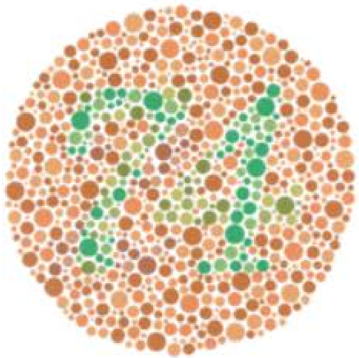


74

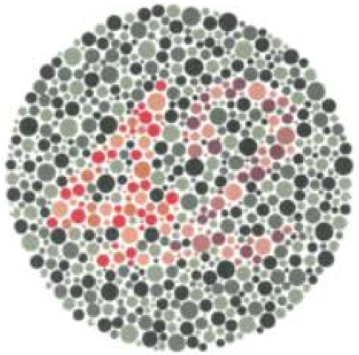

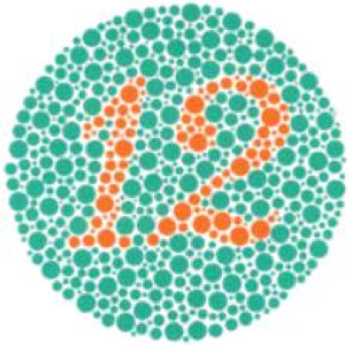


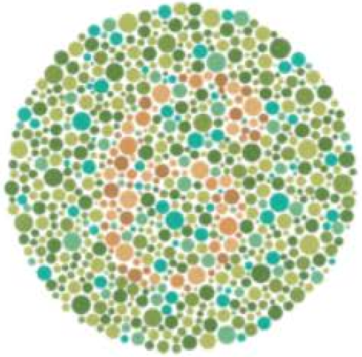

This screening task is to check that you can properly view the colors used in this study based on your viewing conditions, monitor, and vision, among other factors.

Submit »

## DIRECTIONS

This test consists of 30 questions designed to see how well you can visualize the rotation of three-dimensional objects. Shown below is an example of the type of question included in the second section.

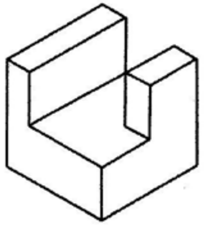

IS ROTATED TO

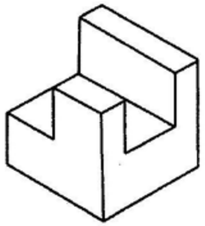

AS

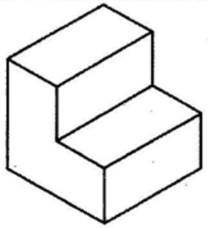

IS ROTATED TO

A

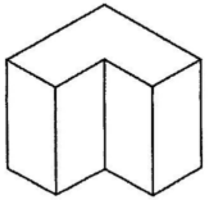

B

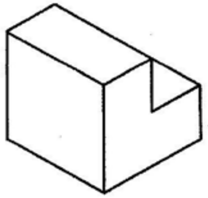

C

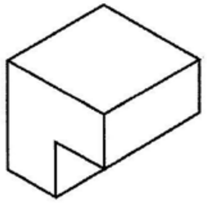

D

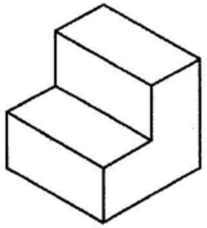

E

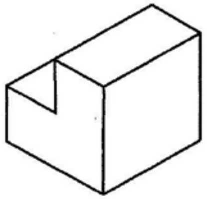

# 30 trials

## (stimuli are copyrighted and can’t be shown here)

https://www.silc.northwestern.edu/revised-purdue-spatial-visualization-test-revised-psvtr-visualization-of-rotations/

Please rate your overall level of confidence in your performance for the previous set of tests.

Low High

The next test is ready.

Begin »

Remaining task types counterbalanced

# Pie Chart Instructions

You will be shown two pie charts.

The two pie charts will use the same color scheme.

A given color represents the same information in both charts (e.g., amount of time spent watching TV in a day).

A slice is unchanged if it is the same size in both charts.The order of the slices does not matter for this task.

Choose whether the two pie charts represent the same data.

This test has a time limit. Your remaining time is indicated at the top of the screen as follows. The practice test has no time limit.

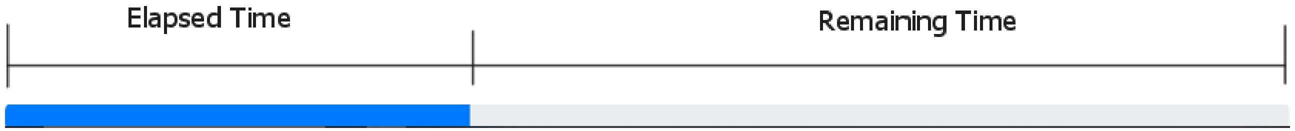


Begin

# Sample Test

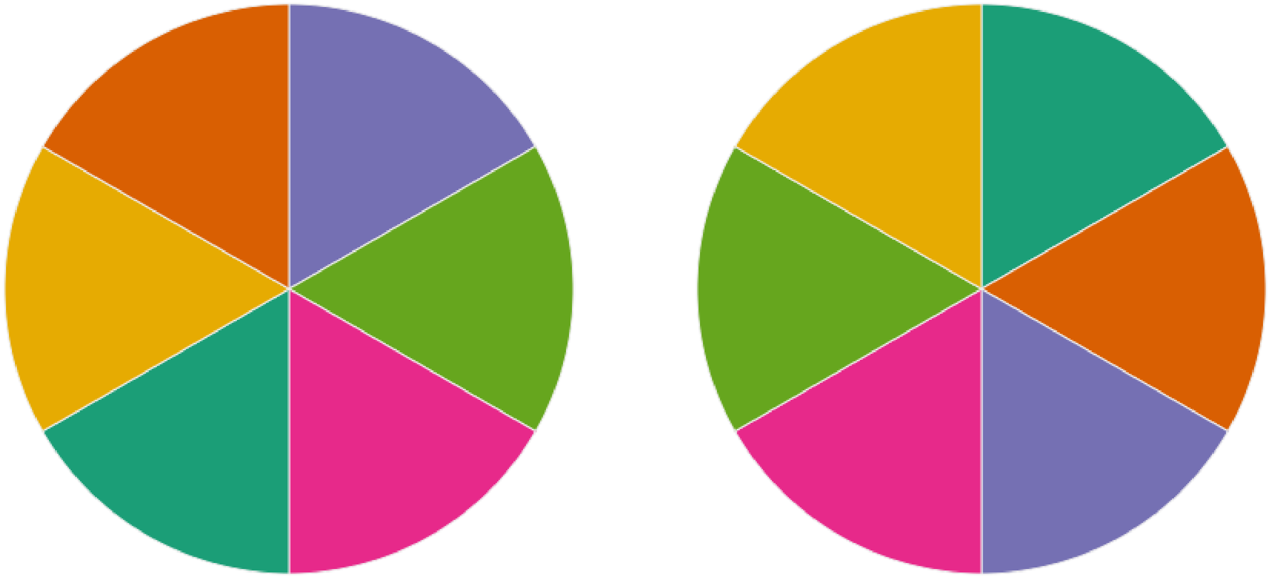

⚠ This is an example of the test you are about to do. Results of this test are not tracked.

Do these pie charts represent the same data?

Yes

No

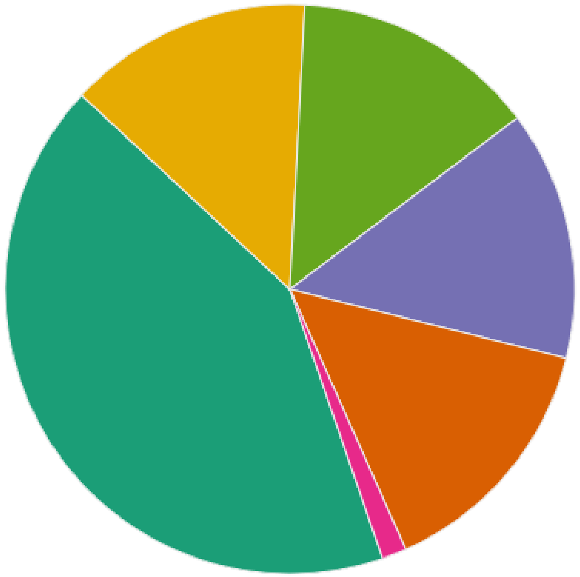

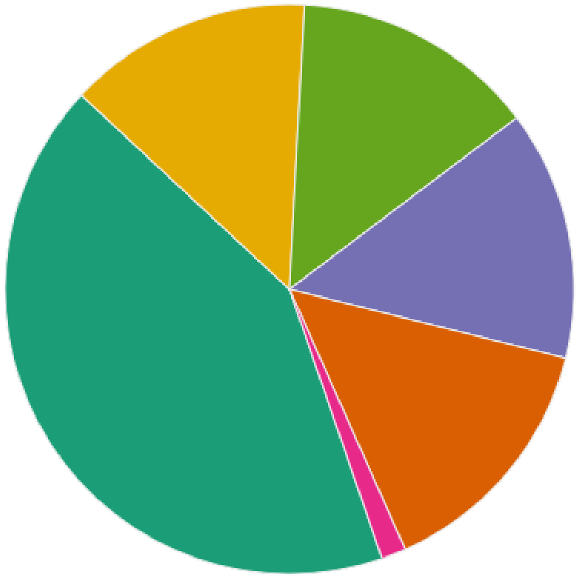

Do these pie charts represent the same data?

Yes

No

# 20 trials

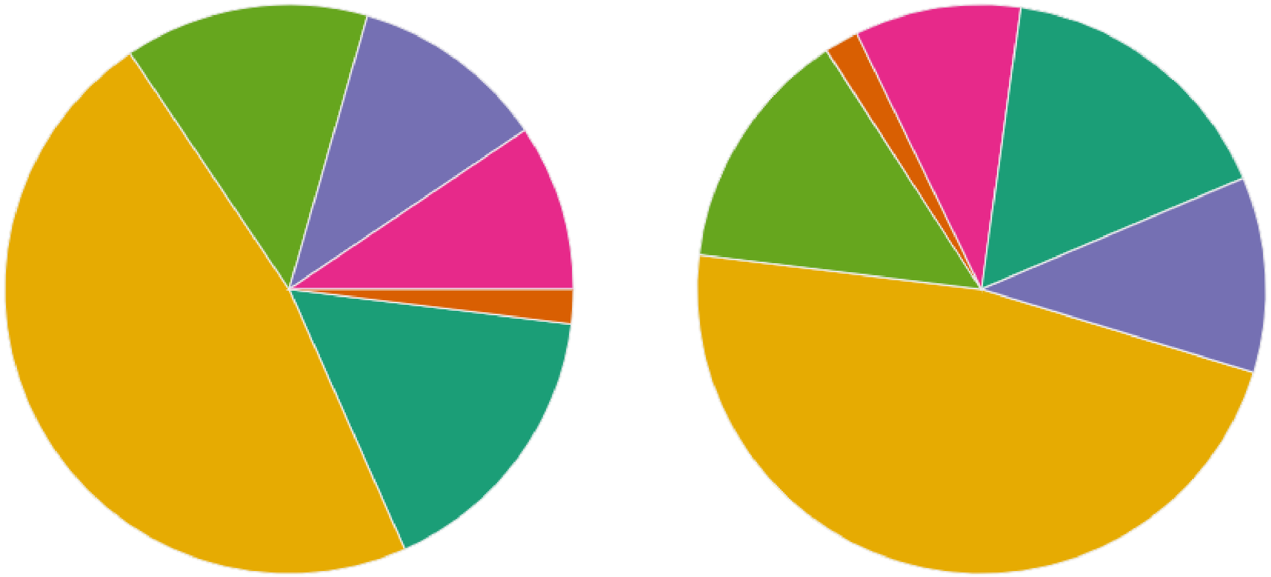

Do these pie charts represent the same data?

Yes

No

Please rate your overall level of confidence in your performance for the previous set of tests.

Low High

The next test is ready.

Begin »

# Isocontour Instructions

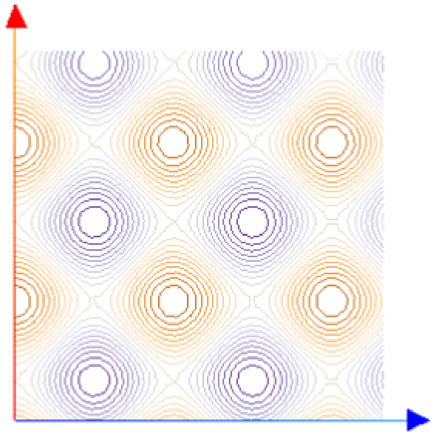

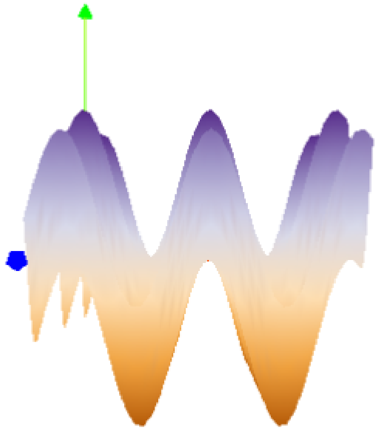

You will be provided with a 2D isocontour (topographical) plot of a 3D surface and a 3D plot (see examples above).

The two plots are the same if they show the same spatial variation along each axis (each arrow).

Choose whether the 2D and 3D plots match each other.

You can rotate the 3D view by clicking on it and dragging your mouse.

This test has a time limit. Your remaining time is indicated at the top of the screen as follows. The practice test has no time limit.

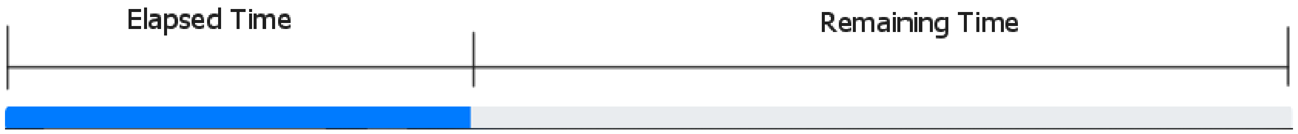


Begin

# Sample Test

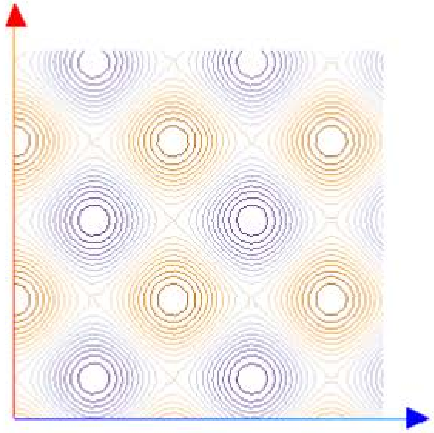

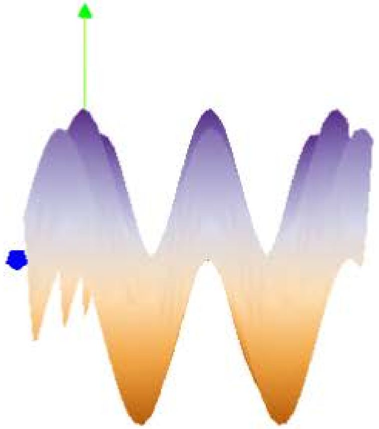

⚠ This is an example of the test you are about to do. Results of this test are not tracked.

Does the 2D plot represent the 3D plot?

Yes

No

# Sample Test

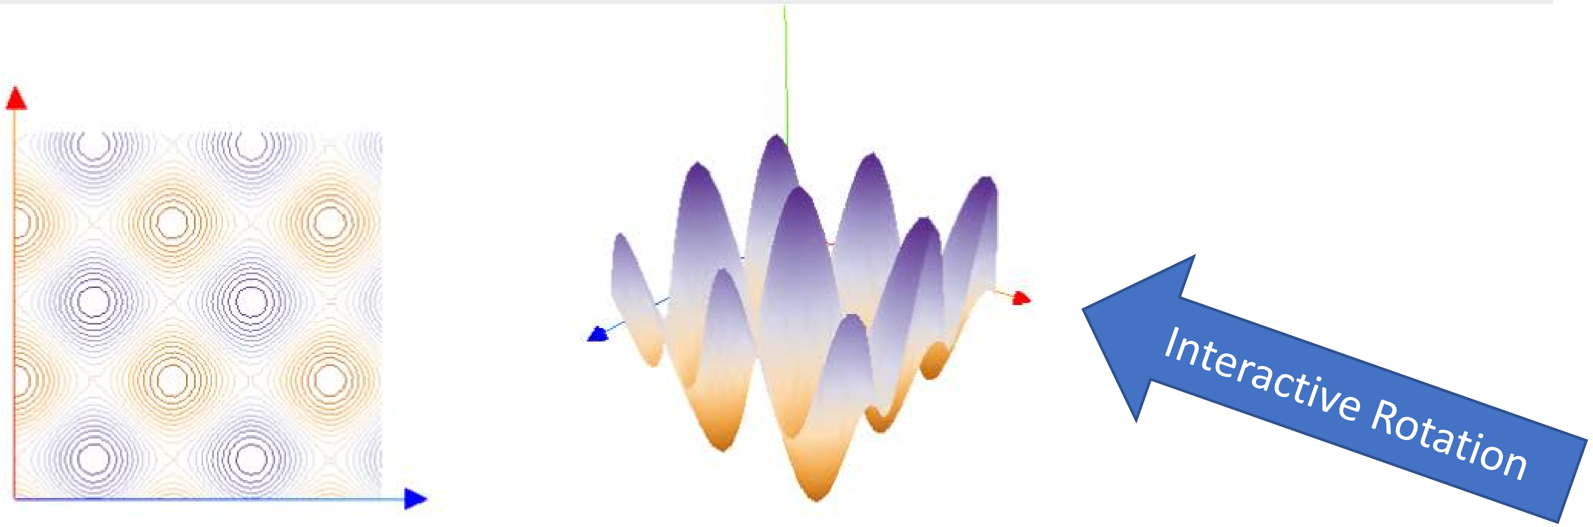


⚠ This is an example of the test you are about to do. Results of this test are not tracked.

Does the 2D plot represent the 3D plot?

Yes | No

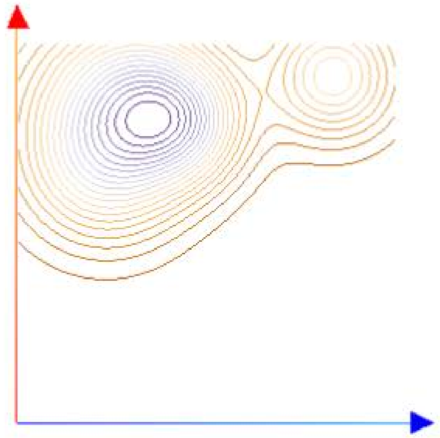

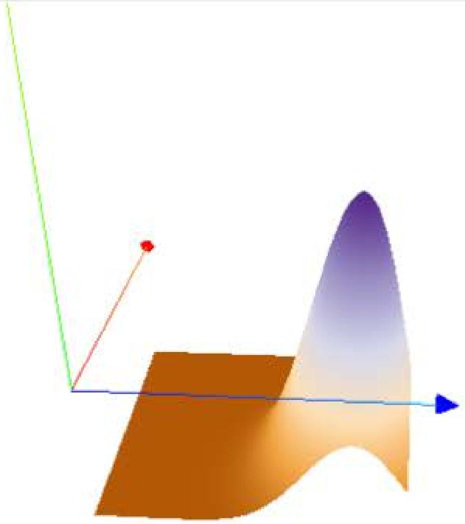

Does the 2D plot represent the 3D plot?

Yes

No

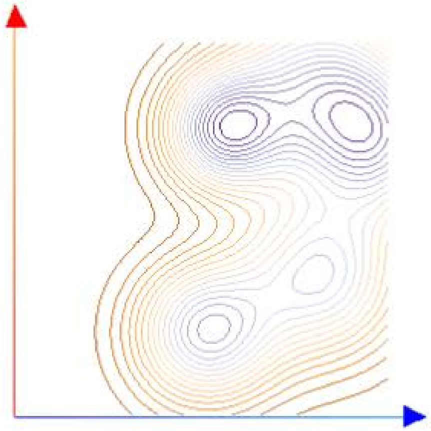

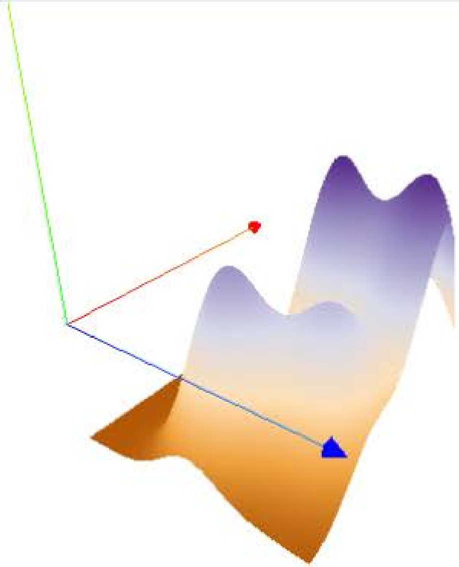

Does the 2D plot represent the 3D plot?

Yes

No

# 20 trials

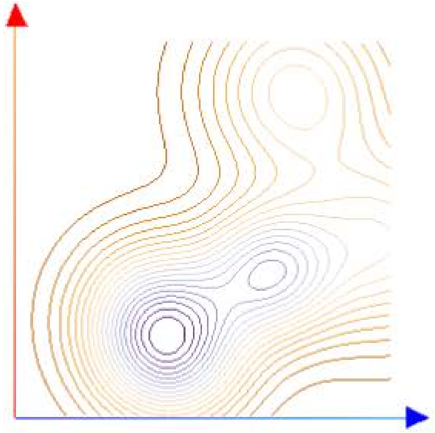

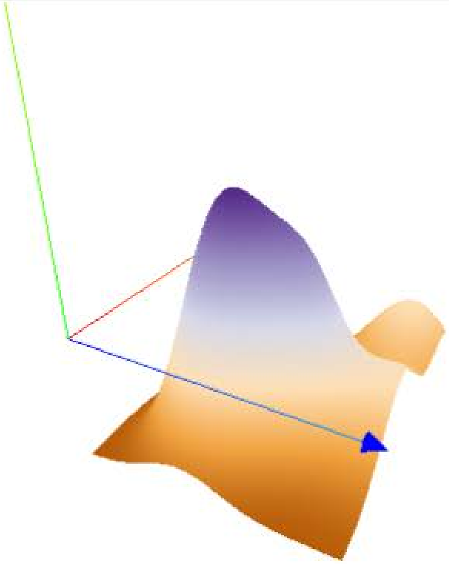

Does the 2D plot represent the 3D plot?

Yes

No

Please rate your overall level of confidence in your performance for the previous set of tests.

Low High

The next test is ready.

Begin »

# Scatter Plot Instructions

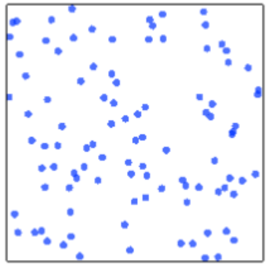

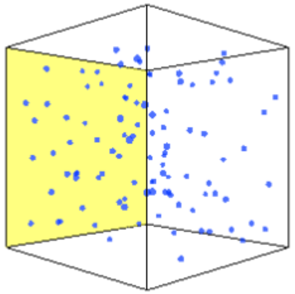

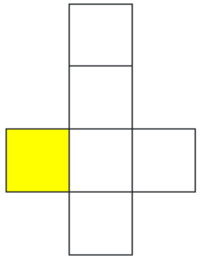

You will be shown a 2D view of a 3D scatter plot, and the corresponding 3D scatter plot.

Choose the side of the 3D scatter plot corresponding to the 2D view.

You can rotate the 3D view by clicking on it and dragging your mouse.

The amount which you are allowed to rotate the 3D view is limited.

Hovering your mouse on a square of the unfolded cube will highlight the corresponding side in the 3D view.

Click that the unfolded square to select it.

You will be shown a 2D view of a 3D scatter plot, and the corresponding 3D scatter plot.

Choose the side of the 3D scatter plot corresponding to the 2D view.

You can rotate the 3D view by clicking on it and dragging your mouse.

The amount which you are allowed to rotate the 3D view is limited.

Hovering your mouse on a square of the unfolded cube will highlight the corresponding side in the 3D view.

Click that the unfolded square to select it.

# Sample Test

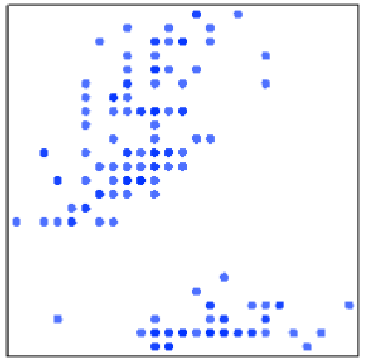

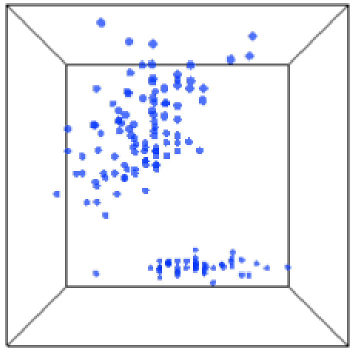

⚠ This is an example of the test you are about to do. Results of this test are not tracked.

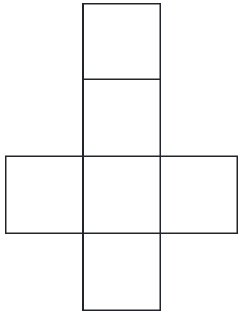

Submit »

# Sample Test

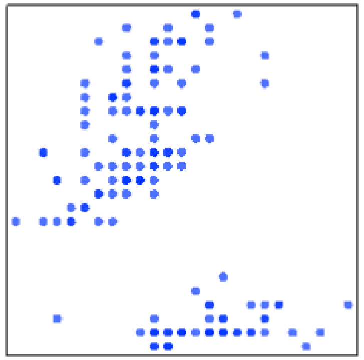

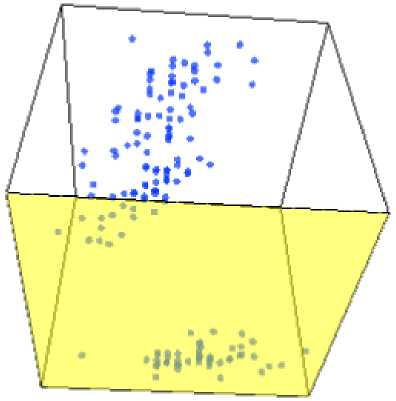

⚠ This is an example of the test you are about to do. Results of this test are not tracked.

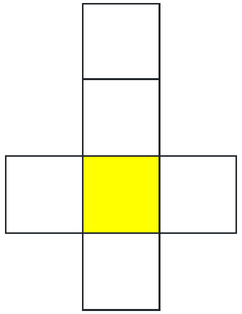

Submit »

# Sample Test

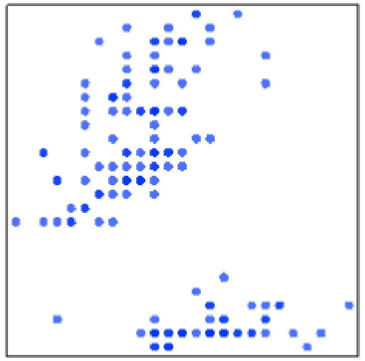

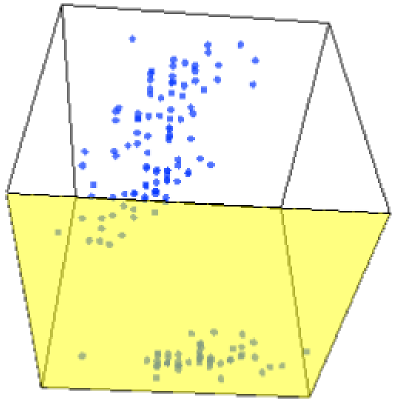

Your answer was correct

Next

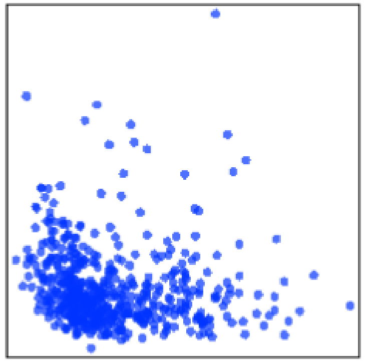

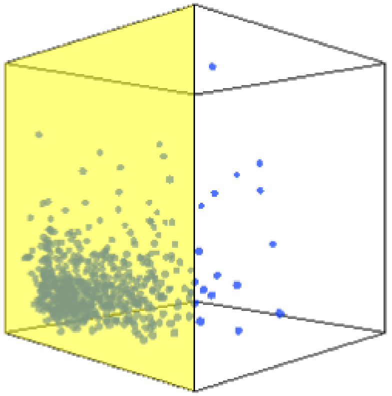

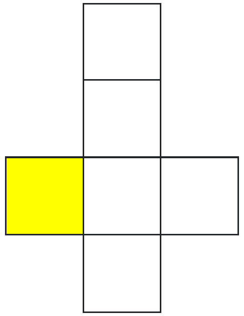

Submit »

10 trials

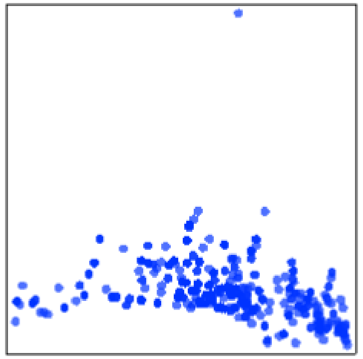

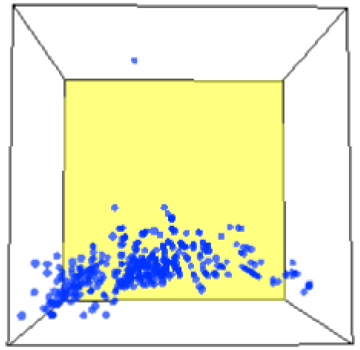

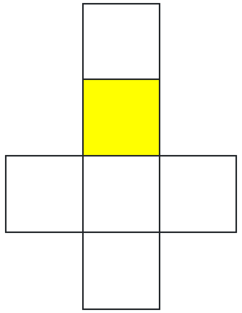

Submit »

Please rate your overall level of confidence in your performance for the previous set of tests.

Low High

The next test is ready.

Begin »

Please describe any strategies that you used to solve each type of test or task.

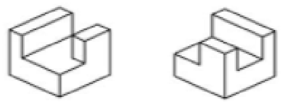

3D Rotation

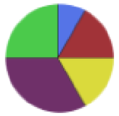

Pie Chart Comparison

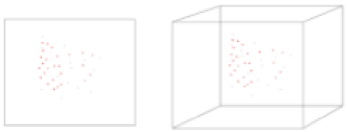

Scatter Plot

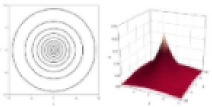

Isocontour

Submit »
